# Supplementary material for: An Inverse Probability Weighted Regression Method that Accounts for Right-censoring for Causal Inference with Multiple Treatments and a Binary Outcome
Source: arXiv:2205.08052 ancillary file (2022-05-17)
Supplement: Supplementary file 1 [file Supplementary_Materials.pdf]

# Supplementary Material to *An Inverse Probability Weighted Regression Method that Accounts for Right-censoring for Causal Inference with Multiple Treatments and a Binary Outcome*

Youfei Yu, Min Zhang*, Bhramar Mukherjee

*Department of Biostatistics, School of Public Health, University of Michigan,*
1415 Washington Heights, Ann Arbor, MI 48109, USA

*mzhangst@umich.edu

## A Derivation of the Asymptotic Distribution of $\hat{\mu}_j$

### A.1 Notations

We first list the notations used in the proof. Let $i$ index the subject and $j$ index the treatment group, with $i = 1, \cdots, n$ and $j = 1, \cdots, J$. Same as the notations in the manuscript, $\tilde{\boldsymbol{X}}_i$, $Z_i$, $T_i$, and $C_i$ denote the covariates, treatment received, time to event, and censoring time, respectively. Let $\Delta_i = I(T_i \leq C_i)$, $R_i = I\{C_i \geq \min(T_i, d)\}$, and $L_i = \min(T_i, C_i, d)$, where $d$ is a fixed time point. $\boldsymbol{V}_i$ and $\boldsymbol{W}_i$ are sets of covariates that are associated with treatment assignment and censoring, respectively. The conditional hazard function of $C_i$ given $\boldsymbol{W}_i$ and $Z_i = j$ is denoted by $\lambda_{ij}(t)$. We define

$$D_{ij} = I(Z_i = j)$$

$$\tilde{Y}_i = I(T_i > d)$$

$$\boldsymbol{S}_j^{(q)}(t; \boldsymbol{\gamma}_j) = n^{-1} \sum_{i=1}^{n} Y_{ij}(t) \boldsymbol{W}_i^{\otimes q} \exp(\boldsymbol{W}_i^T \boldsymbol{\gamma}_j) \qquad \boldsymbol{s}_j^{(q)}(t; \boldsymbol{\gamma}_j) = E\{\boldsymbol{S}_j^{(q)}(t; \boldsymbol{\gamma}_j)\}$$

$$\overline{\boldsymbol{W}}_j(t; \boldsymbol{\gamma}_j) = \frac{\boldsymbol{S}_j^{(1)}(t; \boldsymbol{\gamma}_j)}{S_j^{(0)}(t; \boldsymbol{\gamma}_j)} \qquad \overline{\boldsymbol{w}}_j(t; \boldsymbol{\gamma}_j) = \frac{\boldsymbol{s}_j^{(1)}(t; \boldsymbol{\gamma}_j)}{s_j^{(0)}(t; \boldsymbol{\gamma}_j)}$$

$$m_{ij}(\boldsymbol{\beta}_j) = \text{expit}(\boldsymbol{\beta}_j^T \boldsymbol{X}_i)$$

$$\pi_{ij}(\boldsymbol{\alpha}) = \exp(\boldsymbol{\alpha}_j^T \boldsymbol{V}_i) / \sum_{z=1}^{J} \exp(\boldsymbol{\alpha}_z^T \boldsymbol{V}_i), \text{ where } \boldsymbol{\alpha} = (\alpha_1, \cdots, \alpha_J)^T$$

$$d\Lambda_{0j}^*(t) = \frac{E\{dN_{ij}(t)\}}{s_j^{(0)}(t; \boldsymbol{\gamma}_j^*)}$$

$$d\Lambda_{ij}^*(t) = \exp(\boldsymbol{W}_i^T \boldsymbol{\gamma}_j^*) d\Lambda_{0j}^*(t)$$

$$dM_{ij}^*(t) = dN_{ij}(t) - Y_{ij}(t) d\Lambda_{ij}^*(t)$$

with the counting process defined by $N_{ij}(t) = D_{ij} I\{\min(T_i, C_i) \leq t, \Delta_i = 1\}$ and the at-risk process defined by $Y_{ij}(t) = D_{ij} I\{\min(T_i, C_i) \geq t\}$.

## A.2 Model for Treatment Assignment

We consider a multinomial logistic regression model for the treatment assignment, specified as

$$\frac{\log P(Z_i = l | \boldsymbol{V}_i)}{\log P(Z_i = J | \boldsymbol{V}_i)} = \boldsymbol{V}_i^T \boldsymbol{\alpha}_l, \quad l = 1, \cdots, J-1.$$

Under some regularity conditions [1], $\hat{\boldsymbol{\alpha}}_l$ converges in probability to a constant vector $\boldsymbol{\alpha}_l^*$, denoted by $\hat{\boldsymbol{\alpha}}_l \xrightarrow{p} \boldsymbol{\alpha}_l^*$, and

$$n^{1/2}(\hat{\boldsymbol{\alpha}}_l - \boldsymbol{\alpha}_l^*) = \boldsymbol{H}_l^{-1}(\boldsymbol{\alpha}^*) n^{-1/2} \sum_{i=1}^{n} \boldsymbol{V}_i \{D_{il} - \pi_{il}(\boldsymbol{\alpha}^*)\} + o_p(1) \tag{1}$$

where

$$\boldsymbol{H}_l(\boldsymbol{\alpha}^*) = E\left\{\boldsymbol{V}_i \boldsymbol{V}_i^T \pi_{il}(\boldsymbol{\alpha}^*)\left[1 - \pi_{il}(\boldsymbol{\alpha}^*)\right]\right\}.$$

If the model for $P(Z_i = l | \boldsymbol{V}_i)$ where $l = 1, \cdots, J-1$ is correctly specified, $\boldsymbol{\alpha}^*$ equals the truth $\boldsymbol{\alpha}^0$.

## A.3 Model for Censoring

We assume a Cox proportional hazard model for the censoring time hazard, given by

$$\lambda_{ij}(t) \equiv \lambda(t | Z_i = j, \tilde{\boldsymbol{X}}_i) = \lambda_{0j}(t) \exp\left(\boldsymbol{W}_i^T \boldsymbol{\gamma}_j\right), \quad j = 1, \cdots, J$$

Let $\delta$ be the time point that satisfies $P\{\min(T_i, C_i) \geq \delta\} > 0$ for $i = 1, \cdots, n$, which practically is set to the maximum observation time. Lin and Wei [2] showed that under some regularity conditions, $\hat{\boldsymbol{\gamma}}_j \xrightarrow{p} \boldsymbol{\gamma}_j^*$, and $n^{1/2}(\hat{\boldsymbol{\gamma}}_j - \boldsymbol{\gamma}_j^*)$ is asymptotically normal with

$$n^{1/2}(\hat{\boldsymbol{\gamma}}_j - \boldsymbol{\gamma}_j^*) = \boldsymbol{\Omega}_j^{-1}(\boldsymbol{\gamma}_j^*) n^{-1/2} \sum_{i=1}^{n} \boldsymbol{U}_{ij}(\boldsymbol{\gamma}_j^*) + o_p(1), \tag{2}$$

where $\boldsymbol{\Omega}_j(\boldsymbol{\gamma}_j^*) = \int_0^\delta \left\{ \frac{\boldsymbol{s}_j^{(2)}(t;\boldsymbol{\gamma}_j^*)}{s_j^{(0)}(t;\boldsymbol{\gamma}_j^*)} - \overline{\boldsymbol{w}}_j(t;\boldsymbol{\gamma}_j)^{\otimes 2} \right\} E\{Y_{ij}(t)\lambda_{ij}(t)\} dt$ and $\boldsymbol{U}_{ij}(\boldsymbol{\gamma}_j^*) = \int_0^\delta \{\boldsymbol{W}_i - \overline{\boldsymbol{w}}(t;\boldsymbol{\gamma}_j^*)\} dM_{ij}^*(t)$.

$\Lambda_{0j}(t)$ can be estimated by the Breslow estimator, specified as

$$\hat{\Lambda}_{0j}(t;\hat{\boldsymbol{\gamma}}_j) = \int_0^t \frac{\sum_{i=1}^n dN_{ij}(u)}{\sum_{i=1}^n Y_{ij}(u) \exp\{\boldsymbol{W}_i^T \hat{\boldsymbol{\gamma}}_j\}} \tag{3}$$

We make the following decomposition:

$$n^{1/2}\{\hat{\Lambda}_{ij}(t) - \Lambda_{ij}^*(t)\} = n^{1/2}\{\hat{\Lambda}_{ij}(t;\hat{\boldsymbol{\gamma}}_j) - \hat{\Lambda}_{ij}(t;\boldsymbol{\gamma}_j^*)\} \tag{4}$$

$$+ n^{1/2}\{\hat{\Lambda}_{ij}(t;\boldsymbol{\gamma}_j^*) - \Lambda_{ij}^*(t)\} \tag{5}$$

Applying a Taylor series expansion about $\boldsymbol{\gamma}_j^*$ to (4), we have

$$\begin{aligned}(4) &= \int_0^t \{\boldsymbol{W}_i - \overline{\boldsymbol{w}}_j(u;\boldsymbol{\gamma}_j^*)\} d\hat{\Lambda}_{ij}(u;\boldsymbol{\gamma}_j^*) n^{1/2}(\hat{\boldsymbol{\gamma}}_j - \boldsymbol{\gamma}_j^*) + o_p(1) \\ &= \boldsymbol{K}_{ij}^T(t;\boldsymbol{\gamma}_j^*) \boldsymbol{\Omega}^{-1}(\boldsymbol{\gamma}_j^*) n^{-1/2} \sum_{i=1}^{n} \boldsymbol{U}_{ij}(\boldsymbol{\gamma}_j^*) + o_p(1)\end{aligned}$$

where $\boldsymbol{K}_{ij}(t;\boldsymbol{\gamma}_j^*) = \int_0^t \{\boldsymbol{W}_i - \overline{\boldsymbol{w}}_j(u;\boldsymbol{\gamma}_j^*)\} d\Lambda_{ij}^*(u)$.

Plugging (3) into (5), we can write the second term as

$$\begin{aligned}(5) &= \exp(\boldsymbol{W}_i^T \boldsymbol{\gamma}_j^*) n^{1/2} \{\hat{\Lambda}_{0j}(t;\boldsymbol{\gamma}_j^*) - \Lambda_{0j}^*(t)\} \\ &= \exp(\boldsymbol{W}_i^T \boldsymbol{\gamma}_j^*) n^{-1/2} \sum_{i=1}^n \int_0^t \frac{dM_{ij}^*(u)}{s^{(0)}(u;\boldsymbol{\gamma}_j^*)} + o_p(1)\end{aligned}$$

It follows from the above results that

$$\begin{aligned}n^{1/2}\{\hat{\Lambda}_{ij}(t) - \Lambda_{ij}^*(t)\} =& \boldsymbol{K}_{ij}^T(t;\boldsymbol{\gamma}_j^*) \boldsymbol{\Omega}^{-1}(\boldsymbol{\gamma}_j^*) n^{-1/2} \sum_{i=1}^n \boldsymbol{U}_{ij}(\boldsymbol{\gamma}_j^*) \\ &+ \exp(\boldsymbol{W}_i^T \boldsymbol{\gamma}_j^*) n^{-1/2} \sum_{i=1}^n \int_0^t \frac{dM_{ij}^*(u)}{s^{(0)}(u;\boldsymbol{\gamma}_j^*)} + o_p(1). \end{aligned} \tag{6}$$

## A.4 Model for Outcome

The assumed model for the outcome is

$$\text{logit}\left\{E(\tilde{Y}_i|\tilde{\boldsymbol{X}}_i, Z_i = j)\right\} = \boldsymbol{X}_i^T \boldsymbol{\beta}_j,$$

where estimator for $\boldsymbol{\beta}_j$, denoted by $\hat{\boldsymbol{\beta}}_j$, can be obtained by solving the set of estimating equations

$$0 = n^{-1} \sum_{i=1}^n \frac{D_{ij} R_i \boldsymbol{X}_i \{\tilde{Y}_i - m_{ij}(\hat{\boldsymbol{\beta}}_j)\}}{\pi_{ij}(\hat{\boldsymbol{\alpha}}) \exp\{-\hat{\Lambda}_{ij}(L_i)\}} \equiv G\left(\hat{\boldsymbol{\beta}}_j, \hat{\boldsymbol{\alpha}}_1, \cdots, \hat{\boldsymbol{\alpha}}_{J-1}, \hat{\Lambda}_{ij}(L_i)\right).$$

Under suitable regularity conditions, $\hat{\boldsymbol{\beta}}_j \xrightarrow{p} \boldsymbol{\beta}_j^*$. To obtain the asymptotic distribution of $n^{1/2}(\hat{\boldsymbol{\beta}}_j - \boldsymbol{\beta}_j^*)$, we make the following decomposition:

$$\begin{aligned}n^{1/2}G\left(\hat{\boldsymbol{\beta}}_j, \hat{\boldsymbol{\alpha}}_1, \cdots, \hat{\boldsymbol{\alpha}}_{J-1}, \hat{\Lambda}_{ij}\right) - & n^{1/2}G\left(\boldsymbol{\beta}_j^*, \boldsymbol{\alpha}_1^*, \cdots, \boldsymbol{\alpha}_{J-1}^*, \Lambda_{ij}^*\right) \\ =& n^{1/2}G\left(\hat{\boldsymbol{\beta}}_j, \hat{\boldsymbol{\alpha}}_1, \cdots, \hat{\boldsymbol{\alpha}}_{J-1}, \hat{\Lambda}_{ij}\right) - n^{1/2}G\left(\boldsymbol{\beta}_j^*, \hat{\boldsymbol{\alpha}}_1, \cdots, \hat{\boldsymbol{\alpha}}_{J-1}, \hat{\Lambda}_{ij}\right) \quad (7) \\ &+ n^{1/2}G\left(\boldsymbol{\beta}_j^*, \hat{\boldsymbol{\alpha}}_1, \cdots, \hat{\boldsymbol{\alpha}}_{J-1}, \hat{\Lambda}_{ij}\right) - n^{1/2}G\left(\boldsymbol{\beta}_j^*, \boldsymbol{\alpha}_1^*, \cdots, \hat{\boldsymbol{\alpha}}_{J-1}, \hat{\Lambda}_{ij}\right) \\ &+ \\ &\vdots \qquad (8) \\ &+ n^{1/2}G\left(\boldsymbol{\beta}_j^*, \boldsymbol{\alpha}_1^*, \cdots, \hat{\boldsymbol{\alpha}}_{J-1}, \hat{\Lambda}_{ij}\right) - n^{1/2}G\left(\boldsymbol{\beta}_j^*, \boldsymbol{\alpha}_1^*, \cdots, \boldsymbol{\alpha}_{J-1}^*, \hat{\Lambda}_{ij}\right) \\ &+ n^{1/2}G\left(\boldsymbol{\beta}_j^*, \boldsymbol{\alpha}_1^*, \cdots, \boldsymbol{\alpha}_{J-1}^*, \hat{\Lambda}_{ij}\right) - n^{1/2}G\left(\boldsymbol{\beta}_j^*, \boldsymbol{\alpha}_1^*, \cdots, \boldsymbol{\alpha}_{J-1}^*, \Lambda_{ij}^*\right). \quad (9)\end{aligned}$$

Considering (7), through a Taylor series expansion of $\hat{\boldsymbol{\beta}}_j$ about $\boldsymbol{\beta}_j^*$,

$$(7) = -\boldsymbol{B}_j(\boldsymbol{\beta}_j^*, \boldsymbol{\alpha}^*, \Lambda_{ij}^*) n^{1/2}(\hat{\boldsymbol{\beta}}_j - \boldsymbol{\beta}_j^*) + o_p(1),$$

where

$$\boldsymbol{B}_j(\boldsymbol{\beta}_j^*, \boldsymbol{\alpha}^*, \Lambda_{ij}^*) = E\left[\frac{D_{ij} R_i \boldsymbol{X}_i \boldsymbol{X}_i^T m_{ij}(\boldsymbol{\beta}_j^*)\{1 - m_{ij}(\boldsymbol{\beta}_j^*)\}}{\pi_{ij}(\boldsymbol{\alpha}^*) \exp\{-\Lambda_{ij}^*(L_i)\}}\right].$$

Considering (8), using a Taylor series expansion of $\hat{\boldsymbol{\alpha}}_l$ about $\boldsymbol{\alpha}_l^*$ for $l = 1, \cdots, J-1$, and substituting the results of (1), we have

$$(8) = \boldsymbol{F}_{jl}\left(\boldsymbol{\beta}_j^*, \boldsymbol{\alpha}^*, \Lambda_{ij}^*\right) \boldsymbol{H}_l^{-1}(\boldsymbol{\alpha}^*) n^{-1/2} \sum_{i=1}^n \boldsymbol{V}_i \{D_{il} - \pi_{il}(\boldsymbol{\alpha}^*)\} + o_p(1),$$

where

$$\boldsymbol{F}_{jl}(\boldsymbol{\beta}_j^*, \boldsymbol{\alpha}^*, \Lambda_{ij}^*) = \begin{cases} E\left[\frac{D_{ij} R_i \boldsymbol{X}_i \boldsymbol{V}_i^T \{1 - \pi_{il}^{-1}(\boldsymbol{\alpha}^*)\}\{\tilde{Y}_i - m_{ij}(\boldsymbol{\beta}_j^*)\}}{\exp\{-\Lambda_{ij}^*(L_i)\}}\right] & \text{if} \quad l = j \\ E\left[\frac{D_{ij} R_i \boldsymbol{X}_i \boldsymbol{V}_i^T \exp(\boldsymbol{V}_i^T \boldsymbol{\alpha}_l^*)\{\tilde{Y}_i - m_{ij}(\boldsymbol{\beta}_j^*)\}}{\{D_{iJ} + (1 - D_{iJ})\exp(\boldsymbol{V}_i^T \boldsymbol{\alpha}_j^*)\}\exp\{-\Lambda_{ij}^*(L_i)\}}\right] & \text{if} \quad l \neq j \end{cases}$$

Considering (9), by Taylor series expansion of $\hat{\Lambda}_{ij}(L_i)$ about $\Lambda_{ij}^*(L_i)$, we have

$$(9) = \boldsymbol{P}_j(\boldsymbol{\beta}_j^*, \boldsymbol{\alpha}^*, \Lambda_{ij}^*) \boldsymbol{\Omega}_j^{-1}(\boldsymbol{\gamma}_j^*) n^{-1/2} \sum_{i=1}^n \boldsymbol{U}_{ij}(\boldsymbol{\gamma}_j^*) + \boldsymbol{Q}_j(\boldsymbol{\beta}_j^*, \boldsymbol{\alpha}, \Lambda_{ij}^*) n^{-1/2} \sum_{i=1}^n \int_0^{L_i} \frac{dM_{ij}^*(u)}{s^{(0)}(u; \boldsymbol{\gamma}_j^*)} + o_p(1),$$

where

$$\boldsymbol{P}_j(\boldsymbol{\beta}_j^*, \boldsymbol{\alpha}^*, \Lambda_{ij}^*) = E\left[\frac{D_{ij} R_i \boldsymbol{X}_i \boldsymbol{K}_{ij}^T(L_i; \boldsymbol{\gamma}_j^*)\{\tilde{Y}_i - m_{ij}(\boldsymbol{\beta}_j^*)\}}{\pi_{ij}(\boldsymbol{\alpha}^*)\exp\{-\Lambda_{ij}^*(L_i)\}}\right],$$

$$\boldsymbol{Q}_j(\boldsymbol{\beta}_j^*, \boldsymbol{\alpha}^*, \Lambda_{ij}^*) = E\left[\frac{D_{ij} R_i \boldsymbol{X}_i \exp(\boldsymbol{W}_i^T \boldsymbol{\gamma}_j^*)\{\tilde{Y}_i - m_{ij}(\boldsymbol{\beta}_j^*)\}}{\pi_{ij}(\boldsymbol{\alpha}^*)\exp\{-\Lambda_{ij}^*(L_i)\}}\right]$$

## A.5 Asymptotic Distribution of $\hat{\mu}_j$

For $j = 1, \cdots, J$, through a Taylor series expansion of $\hat{\mu}_j = n^{-1}\sum_{i=1}^n m_{ij}(\hat{\boldsymbol{\beta}}_j)$ about $\boldsymbol{\beta}_j^*$,

$$n^{1/2}(\hat{\mu}_j - \mu_j^0) = n^{-1/2} \sum_{i=1}^n \left\{m_{ij}(\boldsymbol{\beta}_j^*) - \mu_j^0\right\} + \boldsymbol{A}_j(\boldsymbol{\beta}_j^*) n^{1/2}(\hat{\boldsymbol{\beta}}_j - \boldsymbol{\beta}_j^*) + o_p(1),$$

where $\mu_j^0$ is the underlying truth, and

$$\boldsymbol{A}_j(\boldsymbol{\beta}_j^*) = E\left\{\boldsymbol{X}_i^T m_{ij}(\boldsymbol{\beta}_j^*)[1 - m_{ij}(\boldsymbol{\beta}_j^*)]\right\}.$$

Combining the above results, we can represent $n^{1/2}(\hat{\mu}_j - \mu_j^0)$ as $n^{-1/2}\sum_{i=1}^n \psi_{ij} + o_p(1)$, where

$$\begin{aligned}
\psi_{ij} =& m_{ij}(\boldsymbol{\beta}_j^*) - \mu_j^0 + \boldsymbol{A}_j(\boldsymbol{\beta}_j^*)\boldsymbol{B}_j^{-1}(\boldsymbol{\beta}_j^*, \boldsymbol{\alpha}^*, \Lambda_{ij}^*) \frac{D_{ij} R_i \boldsymbol{X}_i \{\tilde{Y}_i - m_{ij}(\boldsymbol{\beta}_j^*)\}}{\pi_{ij}(\boldsymbol{\alpha}^*)\exp\{-\Lambda_{ij}^*(L_i)\}} \\
&+ \boldsymbol{A}_j(\boldsymbol{\beta}_j^*)\boldsymbol{B}_j^{-1}(\boldsymbol{\beta}_j^*, \boldsymbol{\alpha}^*, \Lambda_{ij}^*) \sum_{l=1}^{J-1} \boldsymbol{F}_{jl}\left(\boldsymbol{\beta}_j^*, \boldsymbol{\alpha}^*, \Lambda_{ij}^*\right) \boldsymbol{H}_l^{-1}(\boldsymbol{\alpha}^*) \boldsymbol{V}_i \{D_{il} - \pi_{il}(\boldsymbol{\alpha}^*)\} \\
&+ \boldsymbol{A}_j(\boldsymbol{\beta}_j^*)\boldsymbol{B}_j^{-1}(\boldsymbol{\beta}_j^*, \boldsymbol{\alpha}^*, \Lambda_{ij}^*) \boldsymbol{P}_j(\boldsymbol{\beta}_j, \boldsymbol{\alpha}^*, \Lambda_{ij}^*) \boldsymbol{\Omega}_j^{-1}(\boldsymbol{\gamma}_j^*) \boldsymbol{U}_{ij}(\boldsymbol{\gamma}_j^*) \\
&+ \boldsymbol{A}_j(\boldsymbol{\beta}_j^*)\boldsymbol{B}_j^{-1}(\boldsymbol{\beta}_j^*, \boldsymbol{\alpha}^*, \Lambda_{ij}^*) \boldsymbol{Q}_j(\boldsymbol{\beta}_j^*, \boldsymbol{\alpha}^*, \Lambda_{ij}^*) \int_0^{L_i} \frac{dM_{ij}^*(u)}{s^{(0)}(u; \boldsymbol{\gamma}_j^*)},
\end{aligned}$$

which is commonly referred to as the $i$th influence function of $\hat{\mu}_j$.

## References

[1] George Casella and Roger Berger. *Statistical Inference*. Duxbury Resource Center, June 2001.

[2] D. Y. Lin and L. J. Wei. The Robust Inference for the Cox Proportional Hazards Model. *Journal of the American Statistical Association*, 84(408):1074–1078, December 1989.

# B Supplemental Tables and Figures

Table B.1: Parameter configurations for Setting I of the simulation studies

| | Group 1 | Group 2 | Group 3 |
|---|---|---|---|
| Outcome $(\beta_{0j}, \beta_{1j}, \beta_{2j}, \beta_{3j})$ | | | |
| Weak | (135, 5, 4, 4) | (130, 5, 5, 4) | (125, 5, 6, -5) |
| Strong | (135, 10, 8, 8) | (130, 10, 10, 8) | (125, 10, 12, -10) |
| Censoring $(\gamma_{0j}, \gamma_{1j}, \gamma_{2j}, \gamma_{5j})$ | | | |
| 20% | (-31.1, 0.3, 0.3, 0.3) | (-30.8, -0.2, -0.2, -0.3) | (-30.6, 0.4, 0.3, -0.3) |
| 30% | (-30.55, 0.3, 0.3, 0.3) | (-30.3, -0.2, -0.2, -0.3) | (-30.1, 0.4, 0.3, -0.3) |
| 40% | (-30.2, 0.3, 0.3, 0.3) | (-29.9, -0.2, -0.2, -0.3) | (-29.7, 0.4, 0.3, -0.3) |
| Treatment $(\alpha_{0j}, \alpha_{1j}, \alpha_{2j}, \alpha_{4j})$ | | | |
| | (0, 0, 0, 0) | (0.1, -0.2, -0.2, -0.2) | (-0.08, -0.3, -0.3, 0.2) |

Table B.2: Simulation results for the scenario of random censoring and weak outcome-covariate associations ($n = 1500$) in Setting I. For Pseudo-IPW, (c) denotes a correctly specified propensity model and (m) denotes a misspecified propensity model. For CAIPW-Wang, the first letter and second letter denote the specification of the propensity and outcome model, respectively. For CIPWR and CAIPW-ZS, the first and second letter in the parentheses correspond to the model for coarsening mechanism and outcome, respectively. The outcome model in CAIPW-ZS is always misspecified, and we use c$^*$ to denote the case where the true predictors for the outcome were included in the model. Abbreviations: RMSE, root mean squared error; SD, standard deviation.

| | Bias×1000 | | | Empirical SD×1000 | | | RMSE×1000 | | | Coverage | | |
|---|---|---|---|---|---|---|---|---|---|---|---|---|
| Estimators | 1 vs 2 | 1 vs 3 | 2 vs 3 | 1 vs 2 | 1 vs 3 | 2 vs 3 | 1 vs 2 | 1 vs 3 | 2 vs 3 | 1 vs 2 | 1 vs 3 | 2 vs 3 |
| Naive | 65 | 99 | 35 | 37 | 34 | 36 | 74 | 105 | 50 | 46 | 11 | 74 |
| IPW (c) | 10 | 15 | 6 | 35 | 35 | 34 | 37 | 38 | 35 | 94 | 92 | 94 |
| IPW (m) | 36 | 59 | 23 | 36 | 35 | 35 | 50 | 68 | 42 | 83 | 62 | 90 |
| Pseudo-IPW (c) | -1 | 0 | 0 | 35 | 35 | 35 | 35 | 35 | 35 | 95 | 95 | 95 |
| Pseudo-IPW (m) | 22 | 37 | 16 | 35 | 35 | 36 | 41 | 51 | 39 | 89 | 80 | 92 |
| CAIPW-Wang (c,c) | 1 | 2 | 1 | 36 | 37 | 36 | 36 | 37 | 36 | 95 | 94 | 94 |
| CAIPW-Wang (c,m) | 1 | 2 | 1 | 36 | 37 | 36 | 36 | 37 | 36 | 95 | 94 | 95 |
| CAIPW-Wang (m,c) | 1 | 3 | 2 | 35 | 37 | 37 | 35 | 37 | 37 | 95 | 94 | 94 |
| CIPW (c) | -1 | 0 | 0 | 34 | 35 | 35 | 34 | 35 | 35 | 94 | 95 | 95 |
| CIPW (m) | 22 | 38 | 16 | 35 | 35 | 36 | 41 | 51 | 39 | 90 | 81 | 92 |
| CIPW-ZS (c) | -1 | -1 | 0 | 34 | 35 | 35 | 34 | 35 | 35 | 94 | 95 | 95 |
| CIPW-ZS (m) | 21 | 37 | 16 | 35 | 35 | 36 | 41 | 51 | 39 | 90 | 81 | 92 |
| CAIPW-ZS (c,c$^*$) | -1 | -1 | 0 | 33 | 34 | 34 | 33 | 34 | 34 | 94 | 94 | 94 |
| CAIPW-ZS (c,m) | -1 | -1 | 0 | 33 | 35 | 34 | 33 | 35 | 34 | 94 | 95 | 94 |
| CAIPW-ZS (m,c$^*$) | 2 | 3 | 1 | 33 | 34 | 34 | 33 | 34 | 34 | 94 | 94 | 94 |
| CIPWR (c,c) | -1 | 0 | 1 | 33 | 34 | 34 | 33 | 34 | 34 | 95 | 96 | 96 |
| CIPWR (c,m) | -1 | 0 | 1 | 34 | 35 | 34 | 34 | 35 | 35 | 95 | 96 | 96 |
| CIPWR (m,c) | -1 | 0 | 1 | 33 | 34 | 34 | 33 | 34 | 34 | 95 | 95 | 96 |

Table B.3: Simulation results for the scenario with 20% censoring and weak outcome-covariate associations ($n = 1500$) in Setting I. For Pseudo-IPW, (c) denotes a correctly specified propensity model and (m) denotes a misspecified propensity model. For CAIPW-Wang, the first letter and second letter denote the specification of the propensity and outcome model, respectively. For CIPWR and CAIPW-ZS, the first and second letter in the parentheses correspond to the model for coarsening mechanism and outcome, respectively. The outcome model in CAIPW-ZS is always misspecified, and we use c* to denote the case where the true predictors for the outcome were included in the model. Abbreviations: RMSE, root mean squared error; SD, standard deviation.

| | Bias×1000 | | | Empirical SD×1000 | | | RMSE×1000 | | | Coverage | | |
|---|---|---|---|---|---|---|---|---|---|---|---|---|
| Estimators | 1 vs 2 | 1 vs 3 | 2 vs 3 | 1 vs 2 | 1 vs 3 | 2 vs 3 | 1 vs 2 | 1 vs 3 | 2 vs 3 | 1 vs 2 | 1 vs 3 | 2 vs 3 |
| Naive | 37 | 100 | 63 | 33 | 32 | 33 | 50 | 105 | 71 | 76 | 10 | 44 |
| IPW (c) | 12 | 23 | 10 | 32 | 33 | 32 | 34 | 40 | 34 | 93 | 89 | 94 |
| IPW (m) | 23 | 63 | 40 | 33 | 33 | 33 | 40 | 71 | 52 | 89 | 54 | 78 |
| Pseudo-IPW (c) | -19 | 9 | 28 | 32 | 33 | 33 | 37 | 34 | 43 | 92 | 94 | 86 |
| Pseudo-IPW (m) | 4 | 45 | 41 | 32 | 33 | 34 | 32 | 56 | 53 | 95 | 73 | 77 |
| CAIPW-Wang (c,c) | 7 | 4 | -3 | 31 | 33 | 33 | 32 | 33 | 33 | 94 | 94 | 94 |
| CAIPW-Wang (c,m) | 7 | 4 | -3 | 31 | 33 | 33 | 32 | 33 | 33 | 94 | 95 | 94 |
| CAIPW-Wang (m,c) | -6 | 9 | 15 | 31 | 33 | 33 | 32 | 34 | 36 | 94 | 93 | 92 |
| CIPW (c) | -1 | 1 | 1 | 32 | 34 | 34 | 32 | 34 | 34 | 95 | 95 | 94 |
| CIPW (m) | 13 | 43 | 30 | 32 | 33 | 34 | 35 | 54 | 46 | 93 | 75 | 86 |
| CIPW-ZS (c) | -1 | 0 | 0 | 32 | 33 | 34 | 32 | 33 | 34 | 95 | 95 | 94 |
| CIPW-ZS (m) | 12 | 42 | 30 | 32 | 33 | 34 | 34 | 54 | 45 | 93 | 75 | 85 |
| CAIPW-ZS (c,c*) | -1 | 0 | 1 | 31 | 33 | 33 | 31 | 33 | 33 | 94 | 94 | 94 |
| CAIPW-ZS (c,m) | -1 | 0 | 1 | 31 | 33 | 33 | 31 | 33 | 33 | 94 | 94 | 94 |
| CAIPW-ZS (m,c*) | 2 | 4 | 2 | 31 | 32 | 32 | 31 | 33 | 32 | 95 | 94 | 94 |
| CIPWR (c,c) | -1 | 0 | 1 | 31 | 33 | 33 | 31 | 33 | 33 | 96 | 95 | 95 |
| CIPWR (c,m) | -1 | 1 | 1 | 31 | 33 | 33 | 31 | 33 | 33 | 96 | 96 | 95 |
| CIPWR (m,c) | 2 | 1 | -1 | 31 | 33 | 33 | 31 | 33 | 33 | 95 | 95 | 95 |

Table B.4: Simulation results for the scenario with 30% censoring and weak outcome-covariate associations ($n = 1500$) in Setting I. For Pseudo-IPW, (c) denotes a correctly specified propensity model and (m) denotes a misspecified propensity model. For CAIPW-Wang, the first letter and second letter denote the specification of the propensity and outcome model, respectively. For CIPWR and CAIPW-ZS, the first and second letter in the parentheses correspond to the model for coarsening mechanism and outcome, respectively. The outcome model in CAIPW-ZS is always misspecified, and we use c* to denote the case where the true predictors for the outcome were included in the model. Abbreviations: RMSE, root mean squared error; SD, standard deviation.

| | Bias | | | Empirical SD | | | RMSE | | | Coverage | | |
|---|---|---|---|---|---|---|---|---|---|---|---|---|
| Estimators | 1 vs 2 | 1 vs 3 | 2 vs 3 | 1 vs 2 | 1 vs 3 | 2 vs 3 | 1 vs 2 | 1 vs 3 | 2 vs 3 | 1 vs 2 | 1 vs 3 | 2 vs 3 |
| Naive | 28 | 108 | 80 | 36 | 34 | 36 | 46 | 113 | 87 | 80 | 7 | 26 |
| IPW (c) | 20 | 34 | 13 | 34 | 36 | 35 | 40 | 49 | 37 | 92 | 84 | 93 |
| IPW (m) | 23 | 74 | 50 | 35 | 35 | 35 | 42 | 81 | 61 | 91 | 46 | 70 |
| Pseudo-IPW (c) | -31 | 13 | 44 | 34 | 36 | 36 | 46 | 38 | 56 | 87 | 92 | 76 |
| Pseudo-IPW (m) | -8 | 48 | 56 | 34 | 35 | 36 | 35 | 60 | 67 | 95 | 73 | 65 |
| CAIPW-Wang (c,c) | 35 | 24 | -12 | 35 | 37 | 38 | 49 | 44 | 39 | 82 | 89 | 93 |
| CAIPW-Wang (c,m) | 36 | 24 | -12 | 35 | 37 | 38 | 50 | 44 | 39 | 82 | 89 | 93 |
| CAIPW-Wang (m,c) | 5 | 30 | 25 | 35 | 37 | 37 | 35 | 48 | 45 | 95 | 87 | 90 |
| CIPW (c) | -1 | 2 | 3 | 34 | 38 | 39 | 34 | 39 | 39 | 95 | 94 | 95 |
| CIPW (m) | 6 | 45 | 39 | 34 | 37 | 38 | 35 | 58 | 54 | 95 | 77 | 81 |
| CIPW-ZS (c) | -1 | 0 | 1 | 34 | 37 | 37 | 34 | 37 | 37 | 95 | 94 | 95 |
| CIPW-ZS (m) | 6 | 44 | 39 | 34 | 36 | 37 | 35 | 57 | 54 | 94 | 76 | 81 |
| CAIPW-ZS (c,c*) | -1 | 0 | 1 | 33 | 36 | 36 | 33 | 36 | 36 | 95 | 94 | 94 |
| CAIPW-ZS (c,m) | -1 | 0 | 1 | 33 | 36 | 37 | 33 | 36 | 37 | 95 | 95 | 94 |
| CAIPW-ZS (m,c*) | 1 | 2 | 2 | 33 | 35 | 35 | 33 | 35 | 35 | 95 | 94 | 94 |
| CIPWR (c,c) | -1 | 1 | 1 | 33 | 36 | 37 | 33 | 36 | 37 | 96 | 95 | 95 |
| CIPWR (c,m) | 0 | 2 | 2 | 33 | 37 | 37 | 33 | 37 | 37 | 96 | 95 | 96 |
| CIPWR (m,c) | 4 | 3 | -1 | 33 | 36 | 37 | 33 | 36 | 37 | 95 | 95 | 95 |

Table B.5: Simulation results for the scenario with 40% censoring and weak outcome-covariate associations ($n = 1500$) in Setting I. For Pseudo-IPW, (c) denotes a correctly specified propensity model and (m) denotes a misspecified propensity model. For CAIPW-Wang, the first letter and second letter denote the specification of the propensity and outcome model, respectively. For CIPWR and CAIPW-ZS, the first and second letter in the parentheses correspond to the model for coarsening mechanism and outcome, respectively. The outcome model in CAIPW-ZS is always misspecified, and we use c* to denote the case where the true predictors for the outcome were included in the model. Abbreviations: RMSE, root mean squared error; SD, standard deviation.

| | Bias | | | Empirical SD | | | RMSE | | | Coverage | | |
|---|---|---|---|---|---|---|---|---|---|---|---|---|
| Estimators | 1 vs 2 | 1 vs 3 | 2 vs 3 | 1 vs 2 | 1 vs 3 | 2 vs 3 | 1 vs 2 | 1 vs 3 | 2 vs 3 | 1 vs 2 | 1 vs 3 | 2 vs 3 |
| Naive | 23 | 119 | 96 | 40 | 36 | 37 | 46 | 125 | 103 | 82 | 4 | 15 |
| IPW (c) | 31 | 48 | 17 | 37 | 38 | 37 | 48 | 61 | 40 | 87 | 76 | 92 |
| IPW (m) | 26 | 87 | 61 | 38 | 37 | 37 | 46 | 95 | 72 | 90 | 36 | 62 |
| Pseudo-IPW (c) | -44 | 18 | 61 | 37 | 39 | 39 | 57 | 43 | 73 | 79 | 91 | 65 |
| Pseudo-IPW (m) | -20 | 53 | 73 | 37 | 38 | 39 | 42 | 65 | 83 | 92 | 73 | 53 |
| CAIPW-Wang (c,c) | 47 | 33 | -14 | 38 | 42 | 44 | 60 | 53 | 46 | 78 | 87 | 93 |
| CAIPW-Wang (c,m) | 47 | 33 | -14 | 38 | 42 | 44 | 61 | 53 | 46 | 78 | 86 | 93 |
| CAIPW-Wang (m,c) | 6 | 41 | 36 | 38 | 41 | 43 | 39 | 58 | 56 | 94 | 83 | 87 |
| CIPW (c) | 0 | 4 | 4 | 36 | 47 | 48 | 36 | 47 | 48 | 94 | 94 | 94 |
| CIPW (m) | 0 | 49 | 49 | 37 | 42 | 44 | 37 | 65 | 66 | 95 | 77 | 77 |
| CIPW-ZS (c) | -1 | 1 | 2 | 36 | 42 | 43 | 36 | 42 | 43 | 94 | 95 | 94 |
| CIPW-ZS (m) | -1 | 48 | 49 | 37 | 40 | 42 | 37 | 63 | 64 | 95 | 77 | 77 |
| CAIPW-ZS (c,c*) | -1 | 0 | 0 | 35 | 40 | 42 | 35 | 40 | 42 | 94 | 95 | 95 |
| CAIPW-ZS (c,m) | -1 | 0 | 1 | 35 | 41 | 42 | 35 | 41 | 42 | 94 | 95 | 95 |
| CAIPW-ZS (m,c*) | 0 | 1 | 0 | 35 | 39 | 40 | 35 | 39 | 40 | 94 | 95 | 94 |
| CIPWR (c,c) | 0 | 2 | 2 | 36 | 41 | 43 | 36 | 41 | 43 | 95 | 95 | 95 |
| CIPWR (c,m) | 0 | 5 | 5 | 36 | 42 | 44 | 36 | 43 | 44 | 95 | 95 | 94 |
| CIPWR (m,c) | 7 | 6 | -1 | 35 | 41 | 42 | 36 | 41 | 42 | 95 | 95 | 95 |

Table B.6: Simulation results for the scenario of 30% censoring and strong outcome-covariate associations ($n = 1500$) in Setting I. For Pseudo-IPW, (c) denotes a correctly specified propensity model and (m) denotes a misspecified propensity model. For CAIPW-Wang, the first letter and second letter denote the specification of the propensity and outcome model, respectively. For CIPWR and CAIPW-ZS, the first and second letter in the parentheses correspond to the model for coarsening mechanism and outcome, respectively. The outcome model in CAIPW-ZS is always misspecified, and we use c* to denote the case where the true predictors for the outcome were included in the model. Abbreviations: RMSE, root mean squared error; SD, standard deviation.

| | Bias | | | Empirical SD | | | RMSE | | | Coverage | | |
|---|---|---|---|---|---|---|---|---|---|---|---|---|
| Estimators | 1 vs 2 | 1 vs 3 | 2 vs 3 | 1 vs 2 | 1 vs 3 | 2 vs 3 | 1 vs 2 | 1 vs 3 | 2 vs 3 | 1 vs 2 | 1 vs 3 | 2 vs 3 |
| Naive | 37 | 100 | 63 | 33 | 32 | 33 | 50 | 105 | 71 | 76 | 10 | 44 |
| IPW (c) | 12 | 23 | 10 | 32 | 33 | 32 | 34 | 40 | 34 | 93 | 89 | 94 |
| IPW (m) | 23 | 63 | 40 | 33 | 33 | 33 | 40 | 71 | 52 | 89 | 54 | 78 |
| Pseudo-IPW (c) | -19 | 9 | 28 | 32 | 33 | 33 | 37 | 34 | 43 | 92 | 94 | 86 |
| Pseudo-IPW (m) | 4 | 45 | 41 | 32 | 33 | 34 | 32 | 56 | 53 | 95 | 73 | 77 |
| CAIPW-Wang (c,c) | 23 | 15 | -9 | 32 | 34 | 34 | 39 | 37 | 35 | 88 | 92 | 94 |
| CAIPW-Wang (c,m) | 23 | 15 | -9 | 32 | 34 | 34 | 39 | 37 | 35 | 89 | 91 | 94 |
| CAIPW-Wang (m,c) | 4 | 20 | 16 | 32 | 34 | 34 | 32 | 39 | 37 | 94 | 90 | 92 |
| CIPW (c) | -1 | 1 | 1 | 32 | 34 | 34 | 32 | 34 | 34 | 95 | 95 | 94 |
| CIPW (m) | 13 | 43 | 30 | 32 | 33 | 34 | 35 | 54 | 46 | 93 | 75 | 86 |
| CIPW-ZS (c) | -1 | 0 | 0 | 32 | 33 | 34 | 32 | 33 | 34 | 95 | 95 | 94 |
| CIPW-ZS (m) | 12 | 42 | 30 | 32 | 33 | 34 | 34 | 54 | 45 | 93 | 75 | 85 |
| CAIPW-ZS (c,c*) | -1 | 0 | 1 | 31 | 33 | 33 | 31 | 33 | 33 | 94 | 94 | 94 |
| CAIPW-ZS (c,m) | -1 | 0 | 1 | 31 | 33 | 33 | 31 | 33 | 33 | 94 | 94 | 94 |
| CAIPW-ZS (m,c*) | 2 | 4 | 2 | 31 | 32 | 32 | 31 | 33 | 32 | 95 | 94 | 94 |
| CIPWR (c,c) | -1 | 0 | 1 | 31 | 33 | 33 | 31 | 33 | 33 | 96 | 95 | 95 |
| CIPWR (c,m) | -1 | 1 | 1 | 31 | 33 | 33 | 31 | 33 | 33 | 96 | 96 | 95 |
| CIPWR (m,c) | 2 | 1 | -1 | 31 | 33 | 33 | 31 | 33 | 33 | 95 | 95 | 95 |

Table B.7: Simulation results for the setting of crossed hazard functions (Setting II). In this setting, the models for treatment and censoring were correctly specified. The outcome model was always misspecified. Abbreviations: RMSE, root mean squared error; SD, standard deviation.

| | Bias | | | Empirical SD | | | RMSE | | | Coverage | | |
|---|---|---|---|---|---|---|---|---|---|---|---|---|
| Estimators | 1 vs 2 | 1 vs 3 | 2 vs 3 | 1 vs 2 | 1 vs 3 | 2 vs 3 | 1 vs 2 | 1 vs 3 | 2 vs 3 | 1 vs 2 | 1 vs 3 | 2 vs 3 |
| *Scenario 1* | | | | | | | | | | | | |
| Naive | -12 | -66 | -54 | 34 | 36 | 38 | 36 | 75 | 66 | 88 | 40 | 56 |
| IPW | -12 | -67 | -55 | 34 | 36 | 38 | 36 | 76 | 67 | 93 | 52 | 70 |
| Pseudo-IPW | -17 | -55 | -38 | 36 | 38 | 39 | 40 | 67 | 54 | 92 | 65 | 84 |
| CAIPW-Wang | -9 | -38 | -28 | 32 | 33 | 34 | 33 | 50 | 44 | 92 | 77 | 86 |
| CIPW | 0 | -1 | 0 | 37 | 37 | 38 | 37 | 37 | 38 | 95 | 94 | 95 |
| CIPW-ZS | -1 | -2 | -1 | 36 | 37 | 38 | 36 | 37 | 38 | 95 | 94 | 94 |
| CAIPW-ZS | -1 | -2 | -1 | 33 | 33 | 34 | 33 | 33 | 34 | 94 | 94 | 95 |
| CIPWR | 1 | 1 | 0 | 33 | 32 | 34 | 33 | 32 | 34 | 94 | 94 | 94 |
| *Scenario 2* | | | | | | | | | | | | |
| Naive | -31 | -29 | 3 | 33 | 33 | 34 | 46 | 44 | 34 | 80 | 83 | 93 |
| IPW | -23 | -24 | -1 | 32 | 32 | 32 | 40 | 40 | 32 | 88 | 89 | 94 |
| Pseudo-IPW | -7 | -12 | -4 | 32 | 32 | 32 | 33 | 34 | 32 | 94 | 94 | 94 |
| CAIPW-Wang | -5 | -4 | 2 | 28 | 28 | 27 | 28 | 28 | 27 | 93 | 95 | 95 |
| CIPW | -1 | -1 | 0 | 32 | 32 | 32 | 32 | 32 | 32 | 94 | 95 | 94 |
| CIPW-ZS | -1 | -2 | 0 | 32 | 32 | 31 | 32 | 32 | 31 | 94 | 95 | 94 |
| CAIPW-ZS | -1 | -1 | 0 | 29 | 29 | 28 | 29 | 29 | 28 | 98 | 98 | 98 |
| CIPWR | -1 | -1 | 0 | 28 | 28 | 28 | 28 | 28 | 28 | 94 | 95 | 94 |

Table B.8: Number (%) of patients who were censored by a given time point.

| | ER visits ($N = 7678$) | | | All-cause hospitalization ($N = 7709$) | | |
|---|---|---|---|---|---|---|
| | Overall | Due to treatment switch | Due to dropout | Overall | Due to treatment switch | Due to dropout |
| 180 days | 1595 (20.8%) | 716 (44.9%) | 879 (55.1%) | 1879 (24.6%) | 836 (44.1%) | 1061 (55.9%) |
| 270 days | 2107 (27.4%) | 955 (45.3%) | 1152 (54.7%) | 2585 (33.5%) | 1145 (44.3%) | 1440 (55.7%) |
| 360 days | 2503 (32.6%) | 1136 (45.4%) | 1367 (54.6%) | 3129 (40.6%) | 1382 (44.2%) | 1747 (55.8%) |

Table B.9: Crude risks of emergency room (ER) visits and hospitalization ignoring censored patients.

| | ER visits ($N = 7678$) | | | Hospitalization ($N = 7709$) | | |
|---|---|---|---|---|---|---|
| First-line therapy | Number of patients | Number (%) of uncensored patients | At least one ER visit (%)* | Number of patients | Number (%) of uncensored patients | At least one hospitalization record (%)* |
| Within 180 days | | | | | | |
| Docetaxel | 2311 | 1877 (81.2) | 1006 (53.6) | 2320 | 1797 (77.5) | 738 (41.1) |
| Abiraterone | 2757 | 2261 (82.0) | 923 (40.8) | 2766 | 2177 (78.7) | 583 (26.8) |
| Enzalutamide | 2043 | 1586 (77.6) | 632 (39.8) | 2051 | 1503 (73.3) | 344 (22.9) |
| Sipuleucel-T | 567 | 359 (63.3) | 150 (41.8) | 572 | 335 (58.6) | 84 (25.1) |
| Within 270 days | | | | | | |
| Docetaxel | 2311 | 1751 (75.8) | 1132 (64.6) | 2320 | 1623 (70.0) | 849 (52.3) |
| Abiraterone | 2757 | 2070 (75.1) | 1091 (52.7) | 2766 | 1926 (69.6) | 703 (36.5) |
| Enzalutamide | 2043 | 1442 (70.6) | 740 (51.3) | 2051 | 1304 (63.6) | 407 (31.2) |
| Sipuleucel-T | 567 | 308 (54.3) | 168 (54.5) | 572 | 271 (47.4) | 96 (35.4) |
| Within 360 days | | | | | | |
| Docetaxel | 2311 | 1651 (71.4) | 1186 (71.8) | 2320 | 1489 (64.2) | 896 (60.2) |
| Abiraterone | 2757 | 1924 (69.8) | 1230 (63.9) | 2766 | 1731 (62.6) | 797 (46.0) |
| Enzalutamide | 2043 | 1320 (64.6) | 810 (61.3) | 2051 | 1129 (55.0) | 462 (40.9) |
| Sipuleucel-T | 567 | 280 (49.4) | 186 (66.4) | 572 | 231 (40.4) | 106 (45.9) |

*Percentage was calculated using the number of uncensored patients as the denominator.

Table B.10: Characteristics of patients in the four treatment groups of interest. Abbreviations: ASO, Administrative Service Only; REF, reference group; HR, hazard ratio; HMO, Health Maintenance Organization; PPO, Preferred Provider Organization; CHF, congestive heart failure.

| | Total (N=7678) | Docetaxel (N=2311) | Abiraterone (N=2757) | Enzalutamide (N=2043) | Sipuleucel-T (N=567) |
|---|---|---|---|---|---|
| Variable | Count (%) | Count (%) | Count (%) | Count (%) | Count (%) |
| Age | | | | | |
| <65 | 1252 (16.3) | 618 (26.7) | 404 (14.7) | 148 (7.2) | 82 (14.5) |
| 65-74 | 2549 (33.2) | 926 (40.1) | 835 (30.3) | 597 (29.2) | 191 (33.7) |
| ≥75 | 3877 (50.5) | 767 (33.2) | 1518 (55.1) | 1298 (63.5) | 294 (51.9) |
| Race | | | | | |
| White | 5593 (72.8) | 1783 (77.2) | 1975 (71.6) | 1403 (68.7) | 432 (76.2) |
| Black | 1151 (15.0) | 294 (12.7) | 416 (15.1) | 353 (17.3) | 88 (15.5) |
| Other | 934 (12.2) | 234 (10.1) | 366 (13.3) | 287 (14.0) | 47 (8.3) |
| Education level | | | | | |
| High School Diploma or Less | 2165 (28.2) | 650 (28.1) | 769 (27.9) | 613 (30.0) | 133 (23.5) |
| High School Graduate and Less than Bachelor Degree | 4196 (54.6) | 1260 (54.5) | 1484 (53.8) | 1130 (55.3) | 322 (56.8) |
| Bachelor Degree Plus | 1317 (17.2) | 401 (17.4) | 504 (18.3) | 300 (14.7) | 112 (19.8) |
| Household income range | | | | | |
| <50k | 2443 (31.8) | 687 (29.7) | 856 (31.0) | 746 (36.5) | 154 (27.2) |
| 50k-100k | 3122 (40.7) | 929 (40.2) | 1133 (41.1) | 830 (40.6) | 230 (40.6) |
| >100k | 2113 (27.5) | 695 (30.1) | 768 (27.9) | 467 (22.9) | 183 (32.3) |
| Geographic Region | | | | | |
| South Atlantic | 1917 (25.0) | 551 (23.8) | 681 (24.7) | 548 (26.8) | 137 (24.2) |
| New England | 333 (4.4) | 108 (4.7) | 134 (4.9) | 82 (4.0) | 9 (1.6) |
| Middle Atlantic | 668 (8.7) | 194 (8.4) | 235 (8.5) | 181 (8.9) | 58 (10.2) |
| East North Central | 1242 (16.2) | 382 (16.5) | 455 (16.5) | 307 (15.0) | 98 (17.3) |
| East South Central | 278 (3.6) | 104 (4.5) | 83 (3.0) | 62 (3.0) | 29 (5.1) |
| West North Central | 626 (8.2) | 360 (15.6) | 133 (4.8) | 86 (4.2) | 47 (8.3) |
| West South Central | 781 (10.2) | 254 (11.0) | 269 (9.8) | 194 (9.5) | 64 (11.3) |
| Mountain | 791 (10.3) | 206 (8.9) | 267 (9.7) | 238 (11.6) | 80 (14.1) |
| Pacific | 1042 (13.6) | 152 (6.6) | 500 (18.1) | 345 (16.9) | 45 (7.9) |
| Product | | | | | |
| HMO | 10440(13.5) | 324 (14.0) | 378 (13.7) | 309 (14.8) | 36 (6.3) |
| PPO | 541 (7.0) | 163 (7.1) | 205 (7.4) | 138 (6.8) | 35 (6.2) |
| Other | 6097 (79.4) | 1824 (78.9) | 2174 (78.9) | 1603 (78.5) | 496 (87.5) |
| Metastatic (Yes) | 2963 (38.6) | 1116 (48.3) | 1018 (36.9) | 587 (28.7) | 242 (42.7) |
| ASO (Yes) | 979 (12.8) | 381 (16.5) | 364 (13.2) | 164 (8.0) | 70 (12.3) |
| Year of First Prescription | | | | | |
| 2014 | 969 (12.6) | 319 (13.8) | 405 (14.7) | 165 (8.1) | 80 (14.1) |
| 2015 | 1000 (13.0) | 378 (16.4) | 313 (11.4) | 233 (11.4) | 76 (13.4) |
| 2016 | 1117 (14.5) | 419 (18.1) | 317 (11.5) | 290 (14.2) | 91 (16.0) |
| 2017 | 1461 (19.0) | 425 (18.4) | 612 (22.2) | 318 (15.6) | 106 (18.7) |
| 2018 | 1762 (22.9) | 374 (16.2) | 805 (29.2) | 464 (22.7) | 119 (21.0) |
| 2019 | 1369 (17.8) | 396 (17.1) | 305 (11.1) | 573 (28.0) | 95 (16.8) |
| Diabetes | 2248 (29.3) | 579 (25.1) | 770 (27.9) | 740 (36.2) | 159 (28.0) |
| Hypertension | 5490 (71.5) | 1573 (68.1) | 1948 (70.7) | 1557 (76.2) | 412 (72.7) |
| Arrhythmia | 1754 (22.8) | 452 (19.6) | 652 (23.6) | 545 (26.7) | 105 (18.5) |
| CHF | 908 (11.8) | 182 (7.9) | 334 (12.1) | 346 (16.9) | 46 (8.1) |
| Osteoporosis | 393 (5.1) | 63 (2.7) | 144 (5.2) | 129 (6.3) | 57 (10.1) |
| Provider Type | | | | | |
| Medical oncologist | 4707 (61.3) | 1389 (60.1) | 2017 (73.2) | 1177 (57.6) | 124 (21.9) |
| Others | 2971 (38.7) | 922 (39.9) | 740 (26.8) | 866 (42.4) | 443 (78.1) |

Table B.11: Characteristics of patients who were censored vs. who were not censored within different time windows for ER visits. Abbreviations: ASO, Administrative Service Only; REF, reference group; HR, hazard ratio; HMO, Health Maintenance Organization; PPO, Preferred Provider Organization; CHF, congestive heart failure.

| | Count (%) | | | | | |
|---|---|---|---|---|---|---|
| | 180 days | | 270 days | | 360 days | |
| Variable | Uncensored (N=6083) | Censored (N=1595) | Uncensored (N=5571) | Censored (N=2107) | Uncensored (N=5175) | Censored (N=2503) |
| Treatment | | | | | | |
| Docetaxel | 1877 (30.9) | 434 (27.2) | 1751 (31.4) | 560 (26.6) | 1651 (31.9) | 660 (26.4) |
| Abiraterone | 2261 (37.2) | 496 (31.1) | 2070 (37.2) | 687 (32.6) | 1924 (37.2) | 833 (33.3) |
| Enzalutamide | 1586 (26.1) | 457 (28.7) | 1442 (25.9) | 601 (28.5) | 1320 (25.5) | 723 (28.9) |
| Sipuleucel-T | 359 (5.9) | 208 (13.0) | 308 (5.5) | 259 (12.3) | 280 (5.4) | 287 (11.5) |
| Age | | | | | | |
| <65 | 922 (15.2) | 330 (20.7) | 824 (14.8) | 428 (20.3) | 740 (14.3) | 512 (20.5) |
| 65-74 | 2011 (33.1) | 538 (33.7) | 1834 (32.9) | 715 (33.9) | 1699 (32.8) | 850 (34.0) |
| ≥75 | 3150 (51.8) | 727 (45.6) | 2913 (52.3) | 964 (45.8) | 2736 (52.9) | 1141 (45.6) |
| Race | | | | | | |
| White | 4398 (72.3) | 1195 (74.9) | 4012 (72.0) | 1581 (75.0) | 3723 (71.9) | 1870 (74.7) |
| Black | 950 (15.6) | 201 (12.6) | 873 (15.7) | 278 (13.2) | 810 (15.7) | 341 (13.6) |
| Other | 735 (12.1) | 199 (12.5) | 686 (12.3) | 248 (11.8) | 642 (12.4) | 292 (11.7) |
| Education level | | | | | | |
| High School Diploma or Less | 1741 (28.6) | 424 (26.6) | 1605 (28.8) | 560 (26.6) | 1519 (29.4) | 646 (25.8) |
| High School Graduate and Less than Bachelor Degree | 3316 (54.5) | 880 (55.2) | 3048 (54.7) | 1148 (54.5) | 2808 (54.3) | 1388 (55.5) |
| Bachelor Degree Plus | 1026 (16.9) | 291 (18.2) | 918 (16.5) | 399 (18.9) | 848 (16.4) | 469 (18.7) |
| Household income range | | | | | | |
| <50k | 1981 (32.6) | 462 (29.0) | 1838 (33.0) | 605 (28.7) | 1732 (33.5) | 711 (28.4) |
| 50k-100k | 2476 (40.7) | 646 (40.5) | 2271 (40.8) | 851 (40.4) | 2108 (40.7) | 1014 (40.5) |
| >100k | 1626 (26.7) | 487 (30.5) | 1462 (26.2) | 651 (30.9) | 1335 (25.8) | 778 (31.1) |
| Geographic Region | | | | | | |
| South Atlantic | 1551 (25.5) | 366 (22.9) | 1433 (25.7) | 484 (23.0) | 1324 (25.6) | 593 (23.7) |
| New England | 263 (4.3) | 70 (4.4) | 245 (4.4) | 88 (4.2) | 222 (4.3) | 111 (4.4) |
| Middle Atlantic | 524 (8.6) | 144 (9.0) | 479 (8.6) | 189 (9.0) | 444 (8.6) | 224 (8.9) |
| East North Central | 991 (16.3) | 251 (15.7) | 901 (16.2) | 341 (16.2) | 846 (16.3) | 396 (15.8) |
| East South Central | 209 (3.4) | 69 (4.3) | 184 (3.3) | 94 (4.5) | 170 (3.3) | 108 (4.3) |
| West North Central | 503 (8.3) | 123 (7.7) | 467 (8.4) | 159 (7.5) | 438 (8.5) | 188 (7.5) |
| West South Central | 588 (9.7) | 193 (12.1) | 535 (9.6) | 246 (11.7) | 496 (9.6) | 285 (11.4) |
| Mountain | 615 (10.1) | 176 (11.0) | 561 (10.1) | 230 (10.9) | 517 (10.0) | 274 (10.9) |
| Pacific | 839 (13.8) | 203 (12.7) | 766 (13.7) | 276 (13.7) | 718 (13.9) | 324 (12.9) |
| Product | | | | | | |
| HMO | 820 (13.5) | 220 (13.8) | 755 (13.6) | 285 (13.5) | 701 (13.5) | 339 (13.5) |
| PPO | 449 (7.4) | 92 (5.8) | 418 (7.5) | 123 (5.8) | 392 (7.6) | 149 (6.0) |
| Other | 4814 (79.1) | 1283 (80.4) | 4398 (78.9) | 1699 (80.6) | 4082 (78.9) | 2015 (80.5) |
| Metastatic (Yes) | 2332 (38.3) | 631 (39.6) | 2139 (38.4) | 824 (39.1) | 2005 (38.7) | 958 (38.3) |
| ASO (Yes) | 747 (12.3) | 232 (14.5) | 666 (12.0) | 313 (14.9) | 602 (11.6) | 377 (15.1) |
| Year of First Prescription | | | | | | |
| 2014 | 767 (12.6) | 202 (12.7) | 703 (12.6) | 266 (12.6) | 658 (12.7) | 311 (12.4) |
| 2015 | 818 (13.4) | 182 (11.4) | 766 (13.7) | 234 (11.1) | 726 (14.0) | 274 (10.9) |
| 2016 | 935 (15.4) | 182 (11.4) | 871 (15.6) | 246 (11.7) | 831 (16.1) | 286 (11.4) |
| 2017 | 1222 (20.1) | 239 (15.0) | 1139 (20.4) | 322 (15.3) | 1082 (20.9) | 379 (15.1) |
| 2018 | 1532 (25.2) | 230 (14.4) | 1447 (26.0) | 315 (15.0) | 1376 (26.6) | 386 (15.4) |
| 2019 | 809 (13.3) | 560 (35.1) | 645 (11.6) | 724 (34.4) | 502 (9.7) | 867 (34.6) |
| Diabetes | 1823 (30.0) | 425 (26.6) | 1689 (30.3) | 559 (26.5) | 1586 (30.6) | 662 (26.4) |
| Hypertension | 4394 (72.2) | 1096 (68.7) | 4042 (72.6) | 1448 (68.7) | 3781 (73.1) | 1709 (68.3) |
| Arrhythmia | 1441 (23.7) | 313 (19.6) | 1346 (24.2) | 408 (19.4) | 1283 (24.8) | 471 (18.8) |
| CHF | 754 (12.4) | 154 (9.7) | 712 (12.8) | 196 (9.3) | 684 (13.2) | 224 (8.9) |
| Osteoporosis | 307 (5.0) | 86 (5.4) | 280 (5.0) | 113 (5.4) | 271 (5.2) | 122 (4.9) |
| Provider Type | | | | | | |
| Medical oncologist | 3788 (62.3) | 919 (57.6) | 3472 (62.3) | 1235 (57.6) | 3227 (62.4) | 1480 (59.1) |
| Others | 2295 (37.7) | 676 (42.4) | 2099 (37.7) | 872 (41.4) | 1948 (37.6) | 1023 (40.9) |

Table B.12: Treatment-specific log hazard ratios and associated p-values for each covariate from Cox proportional hazard models on censoring time. Abbreviations: ASO, Administrative Service Only; REF, reference group; HR, hazard ratio; HMO, Health Maintenance Organization; PPO, Preferred Provider Organization; CHF, congestive heart failure.

| | Docetaxel | | Abiraterone | | Enzalutamide | | Sipuleucel-T | |
|---|---|---|---|---|---|---|---|---|
| Variable | Log HR | p-value | Log HR | p-value | Log HR | p-value | Log HR | p-value |
| Age (REF: <65) | | | | | | | | |
| 65-74 | -0.29 | <0.01 | -0.19 | 0.03 | -0.36 | <0.01 | 0.01 | 0.96 |
| ≥75 | -0.39 | <0.01 | -0.21 | 0.02 | -0.49 | <0.01 | -0.23 | 0.23 |
| Race (REF: White) | | | | | | | | |
| Black | 0.18 | 0.10 | -0.11 | 0.24 | -0.29 | <0.01 | 0.17 | 0.30 |
| Other | 0.04 | 0.74 | -0.21 | 0.04 | 0.02 | 0.88 | -0.42 | 0.05 |
| Education level (REF: High School Diploma or Less) | | | | | | | | |
| High School Graduate and Less than Bachelor Degree | 0.11 | 0.22 | 0.04 | 0.64 | 0.09 | 0.27 | -0.05 | 0.74 |
| Bachelor Degree Plus | 0.02 | 0.86 | -0.02 | 0.86 | 0.19 | 0.12 | 0.31 | 0.13 |
| Household income range | | | | | | | | |
| 50k-100k | -0.12 | 0.19 | 0.03 | 0.68 | -0.04 | 0.58 | -0.04 | 0.78 |
| >100k | -0.23 | 0.03 | 0.05 | 0.60 | -0.05 | 0.65 | -0.08 | 0.64 |
| Geographic Region (REF: South Atlantic) | | | | | | | | |
| New England | -0.05 | 0.78 | 0.36 | 0.05 | -0.09 | 0.68 | 0.00 | 1.00 |
| Middle Atlantic | 0.13 | 0.33 | 0.22 | 0.06 | 0.08 | 0.52 | -0.15 | 0.50 |
| East North Central | 0.12 | 0.28 | 0.07 | 0.48 | 0.17 | 0.12 | 0.3 | 0.10 |
| East South Central | 0.13 | 0.39 | 0.23 | 0.17 | 0.17 | 0.39 | -0.17 | 0.58 |
| West North Central | -0.26 | 0.04 | 0.07 | 0.61 | -0.31 | 0.1 | 0.26 | 0.33 |
| West South Central | 0.00 | 0.98 | 0.01 | 0.93 | 0.26 | 0.03 | 0.42 | 0.03 |
| Mountain | -0.14 | 0.32 | -0.02 | 0.85 | 0.07 | 0.55 | 0.41 | 0.04 |
| Pacific | -0.06 | 0.69 | -0.01 | 0.95 | -0.19 | 0.14 | 0.17 | 0.47 |
| Product (REF: HMO) | | | | | | | | |
| PPO | -0.24 | 0.18 | -0.20 | 0.22 | -0.04 | 0.84 | 0.72 | 0.04 |
| Other | -0.22 | 0.05 | -0.18 | 0.11 | -0.13 | 0.29 | 0.55 | 0.04 |
| Metastatic (Yes) | 0.19 | <0.01 | 0.03 | 0.67 | 0.27 | <0.01 | 0.13 | 0.35 |
| ASO (Yes) | -0.03 | 0.78 | 0.20 | 0.02 | 0.01 | 0.97 | 0.15 | 0.42 |
| Year of First Prescription (REF: 2014) | | | | | | | | |
| 2015 | -0.03 | 0.82 | -0.30 | 0.01 | 0.26 | 0.12 | -0.39 | 0.09 |
| 2016 | -0.01 | 0.92 | -0.26 | 0.03 | -0.07 | 0.67 | -0.24 | 0.27 |
| 2017 | 0.20 | 0.12 | -0.15 | 0.16 | 0.26 | 0.1 | 0.33 | 0.13 |
| 2018 | 0.60 | <0.01 | 0.12 | 0.23 | 0.58 | <0.01 | 0.14 | 0.49 |
| 2019 | 1.72 | <0.01 | 1.27 | <0.01 | 2.10 | <0.01 | 0.8 | <0.01 |
| Diabetes | -0.06 | 0.50 | -0.04 | 0.62 | -0.01 | 0.90 | -0.16 | 0.23 |
| Hypertension | -0.04 | 0.57 | 0.02 | 0.79 | 0.01 | 0.88 | 0.18 | 0.17 |
| Arrhythmia | 0.10 | 0.32 | -0.06 | 0.50 | -0.12 | 0.17 | 0.02 | 0.91 |
| CHF | 0.07 | 0.65 | 0.24 | 0.05 | -0.06 | 0.60 | -0.13 | 0.66 |
| Osteoporosis | 0.07 | 0.74 | -0.14 | 0.34 | 0.05 | 0.70 | -0.24 | 0.25 |
| Provider Type (REF: Medical oncologist) | | | | | | | | |
| Others | -0.06 | 0.46 | 0.04 | 0.50 | 0.11 | 0.11 | -0.24 | 0.10 |

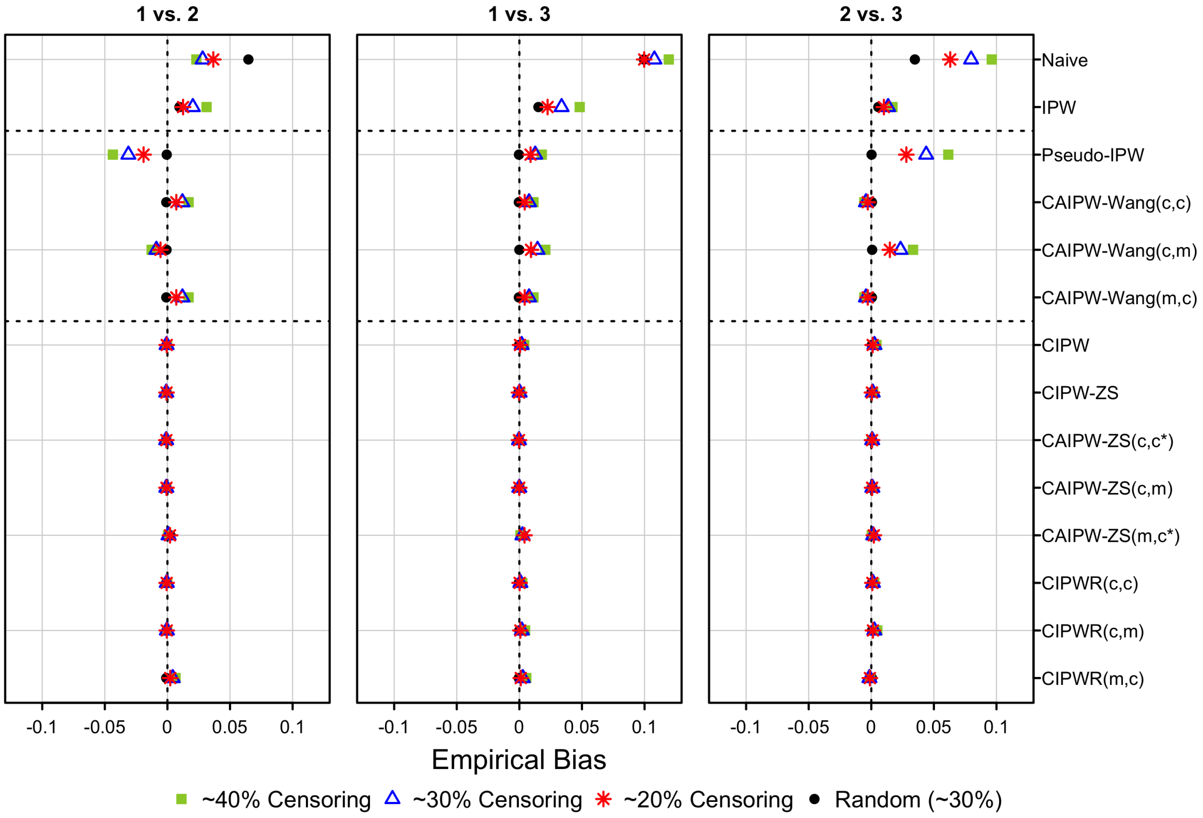


Figure B.1: Empirical bias for different proportions of censoring in Setting I. For CAIPW-Wang, the first letter and second letter denote the specification of the propensity and outcome model, respectively. For CIPWR and CAIPW-ZS, the first and second letter in the parentheses correspond to the model for coarsening mechanism and outcome, respectively. The outcome model in CAIPW-ZS is always misspecified, and we use $c^*$ to denote the case where the true predictors for the outcome were included in the model. Propensity model is correctly specified for IPW, Pseudo-IPW, CIPW, and CIPW-ZS. Sample size was 1500. Results were obtained using 2000 simulated datasets.

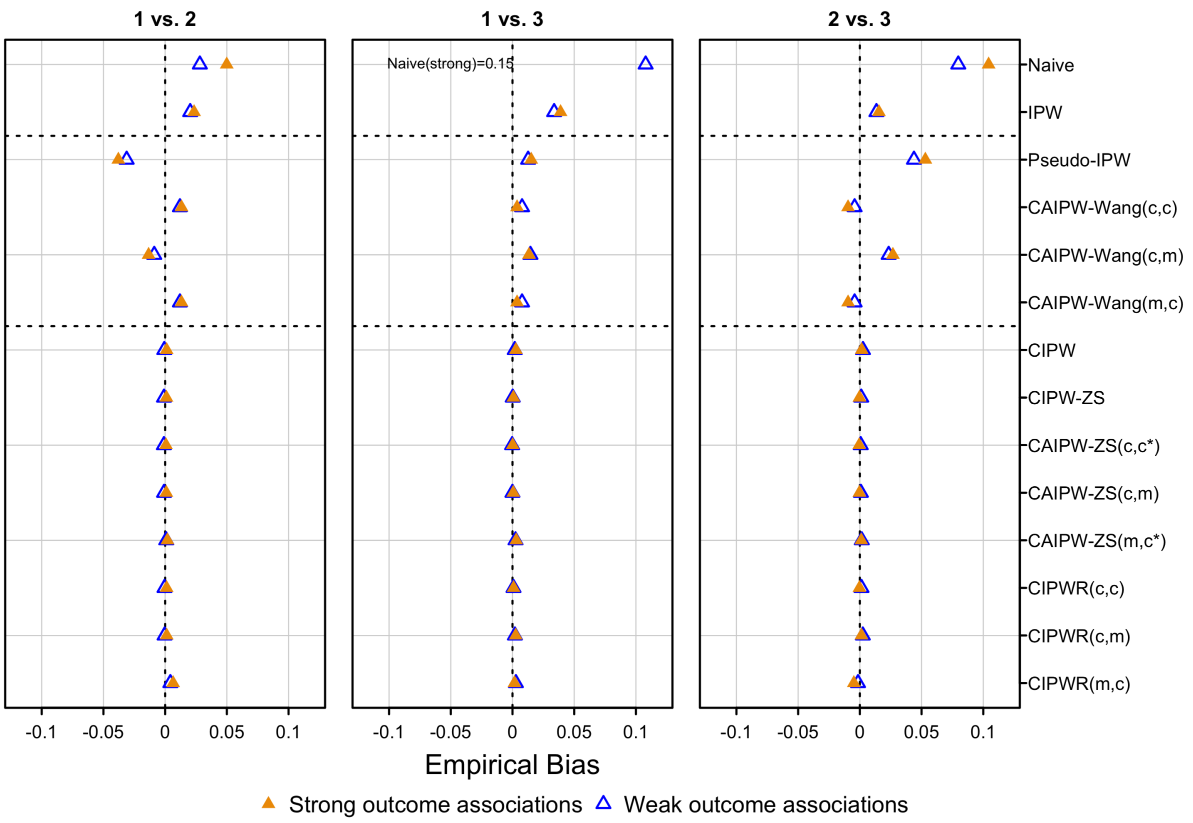


Figure B.2: Empirical bias for different levels of outcome-covariate associations in Setting I. Censoring depended on covariates and the proportion of censoring at $d = 130$ was 30%. For CAIPW-Wang, the first letter and second letter denote the specification of the propensity and outcome model, respectively. For CIPWR and CAIPW-ZS, the first and second letter in the parentheses correspond to the model for coarsening mechanism and outcome, respectively. The outcome model in CAIPW-ZS is always misspecified, and we use c* to denote the case where the true predictors for the outcome were included in the model. Propensity model is correctly specified for IPW, Pseudo-IPW, CIPW, and CIPW-ZS. Sample size was 1500. Results were obtained using 2000 simulated datasets.

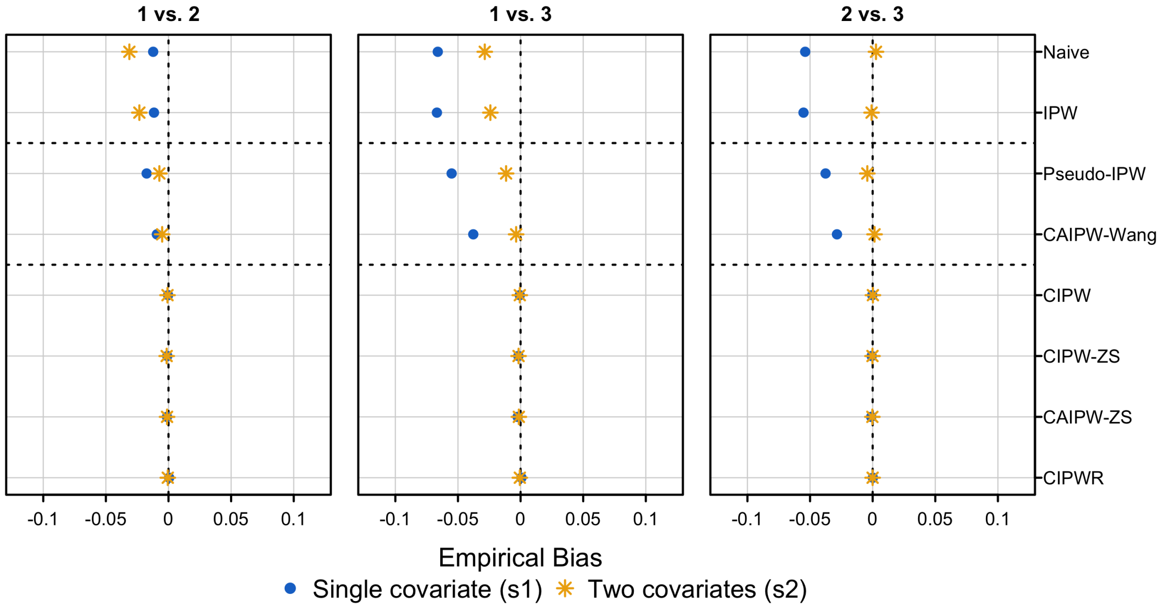


Figure B.3: Empirical bias in the setting of nonproportional hazards (Setting II). The models for treatment assignment and censoring were correctly specified. The logistic regression model and Cox model for the outcome were always misspecified in this setting. Numbers that fall outside the range of x-axis are labeled in the figure. Sample size was 1500. Results were obtained using 2000 simulated datasets.

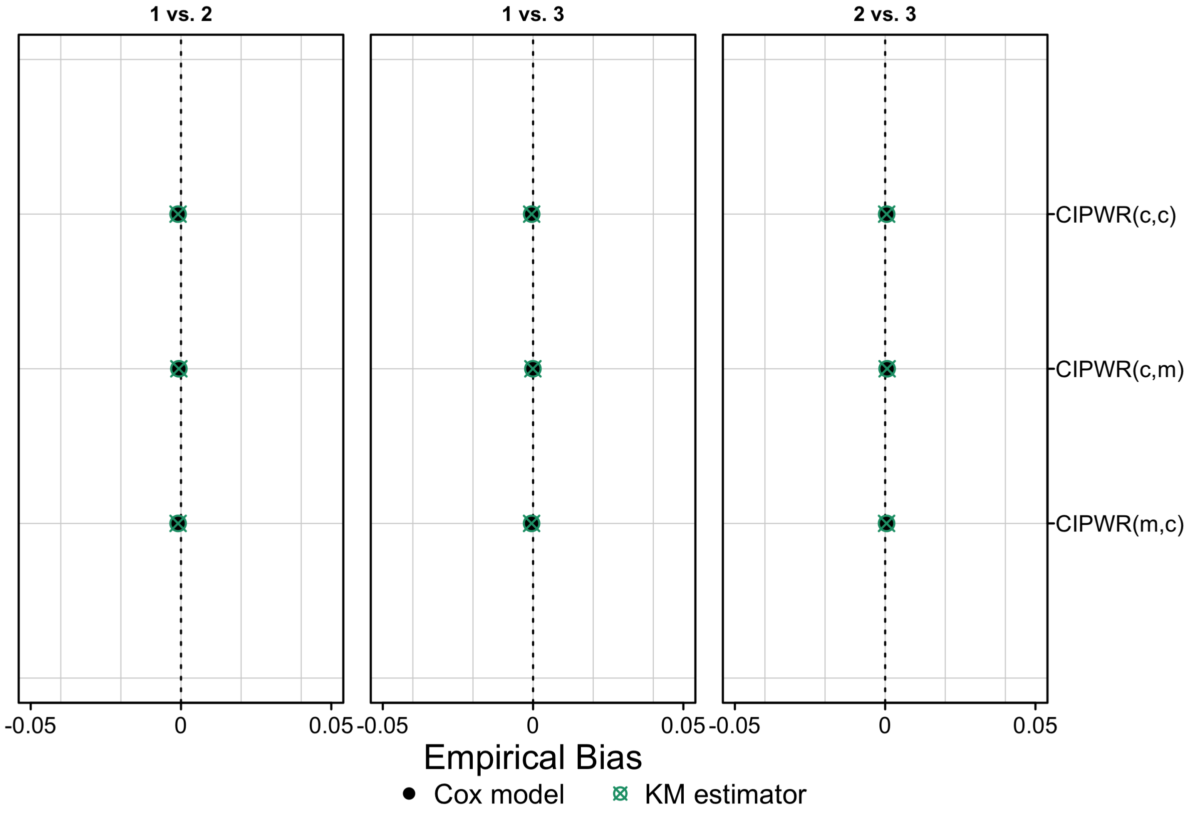


Figure B.4: Empirical bias for CIPWR using Cox model or Kaplan-Meier estimator for estimating censoring probability. The first and second letter in the parentheses correspond to the model for coarsening mechanism and outcome, respectively. Sample size was 1500. Results were obtained using 2000 simulated datasets.

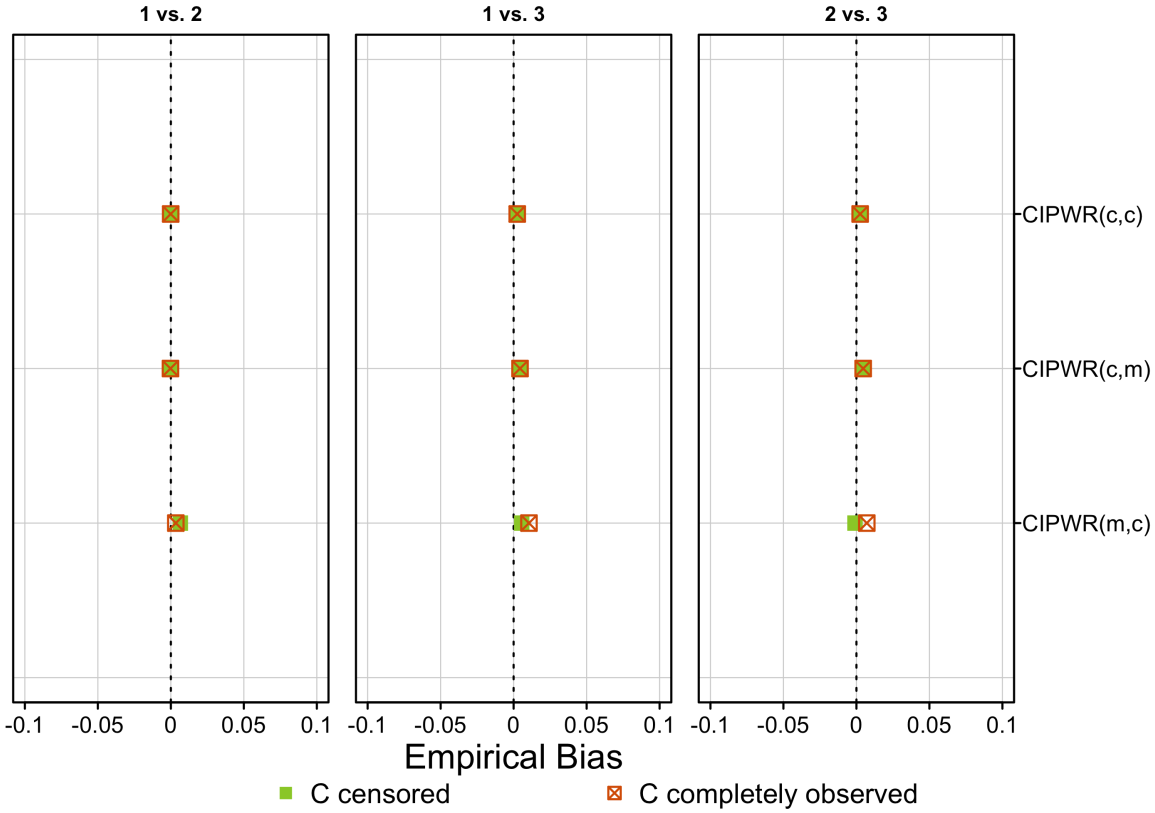


Figure B.5: Empirical bias for Cox model-based CIPWR using observed censoring time or observation time. The first and second letter in the parentheses correspond to the model for coarsening mechanism and outcome, respectively. Sample size was 1500. Results were obtained using 2000 simulated datasets.

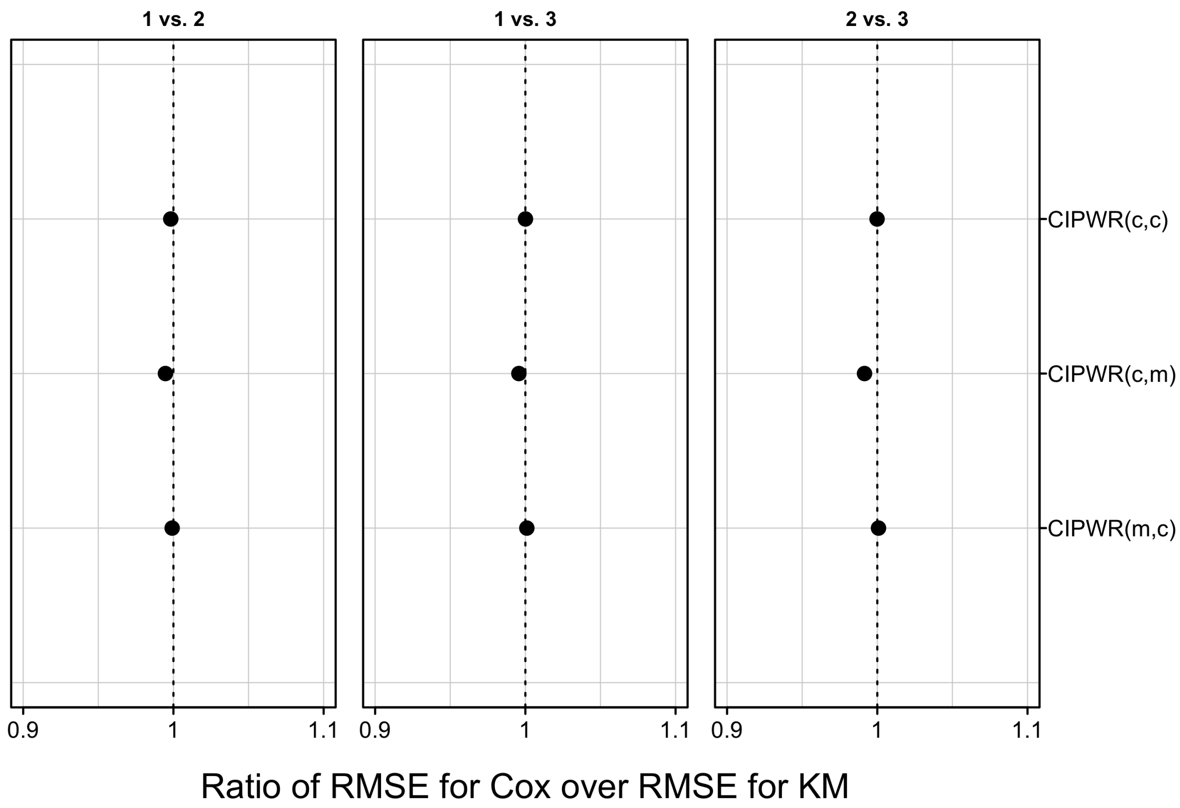


Figure B.6: RMSE for CIPWR using Cox model over RMSE for CIPWR using Kaplan-Meier estimator for estimating censoring probability. The first and second letter in the parentheses correspond to the model for coarsening mechanism and outcome, respectively. Sample size was 1500. Results were obtained using 2000 simulated datasets.

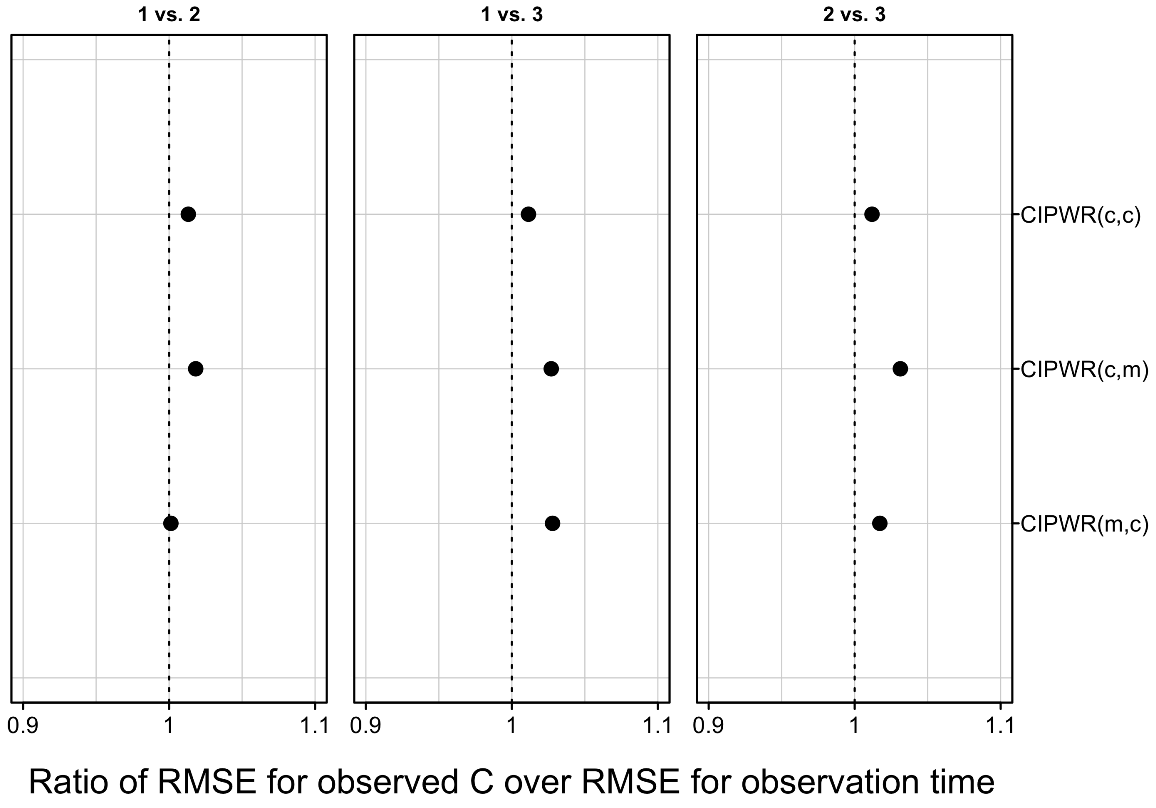


Figure B.7: RMSE for CIPWR using observed censoring time over RMSE for CIPWR using observation time for estimating censoring probability. The first and second letter in the parentheses correspond to the model for coarsening mechanism and outcome, respectively. Sample size was 1500. Results were obtained using 2000 simulated datasets.

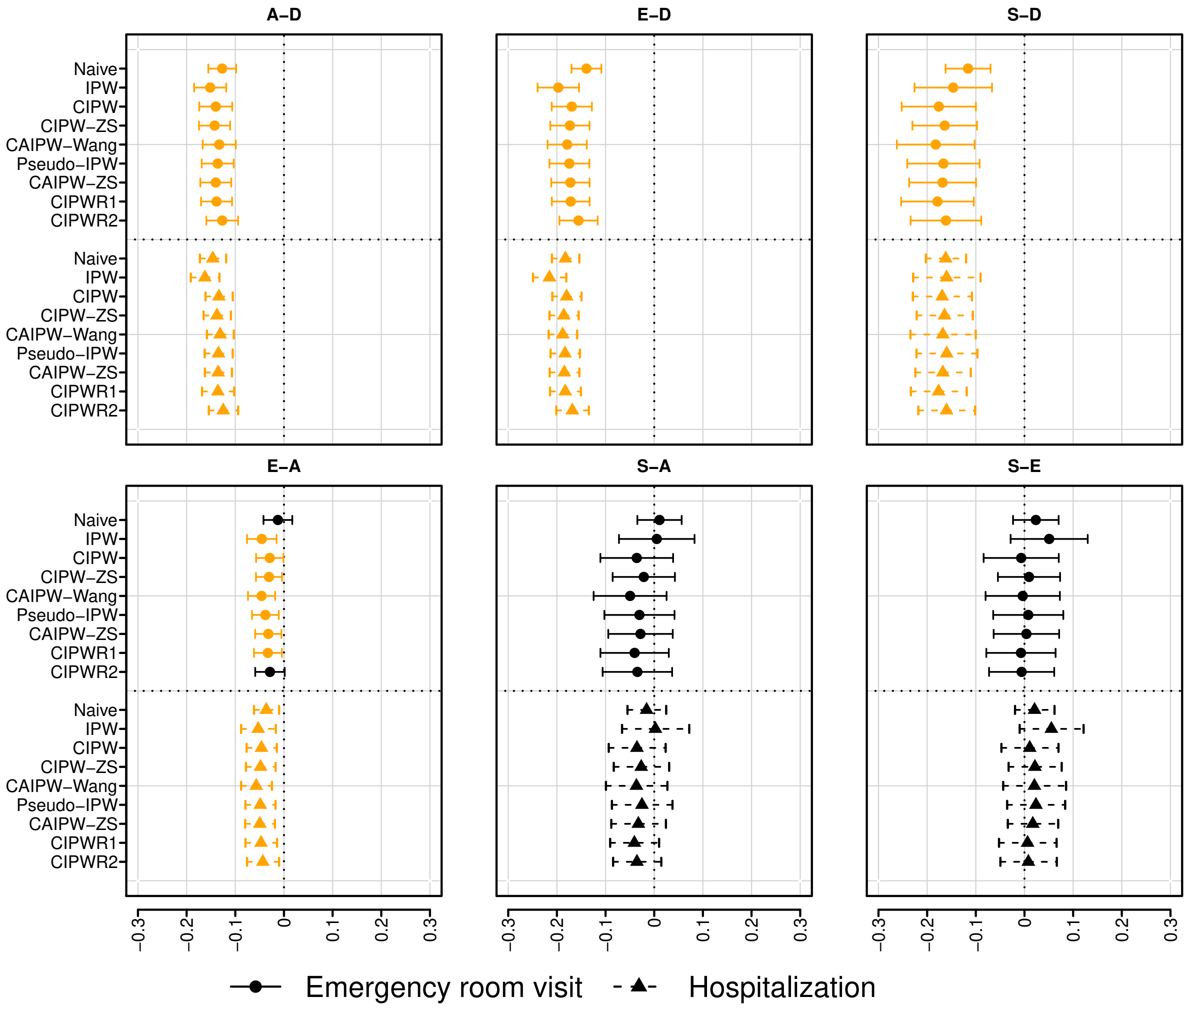


Figure B.8: Average treatment effects for ER visits and hospitalization within 180 days of treatment initiation. Data were obtained from Optum Clinformative Data Mart. Total sample size was $N = 7003$ ($N_A = 2458$, $N_D = 2162$, $N_E = 1833$, $N_S = 550$) for ER visits, and $N = 7045$ ($N_A = 2474$, $N_D = 2172$, $N_E = 1843$, $N_S = 556$) for hospitalization. CIPWR1 is based on observation time, and CIPWR2 is based on observed censoring time. Confidence intervals that exclude zero are highlighted in orange. Abbreviations: A, abiraterone; D, docetaxel; E, enzalutamide; S, sipuleucel-T; ER, emergency room visit.

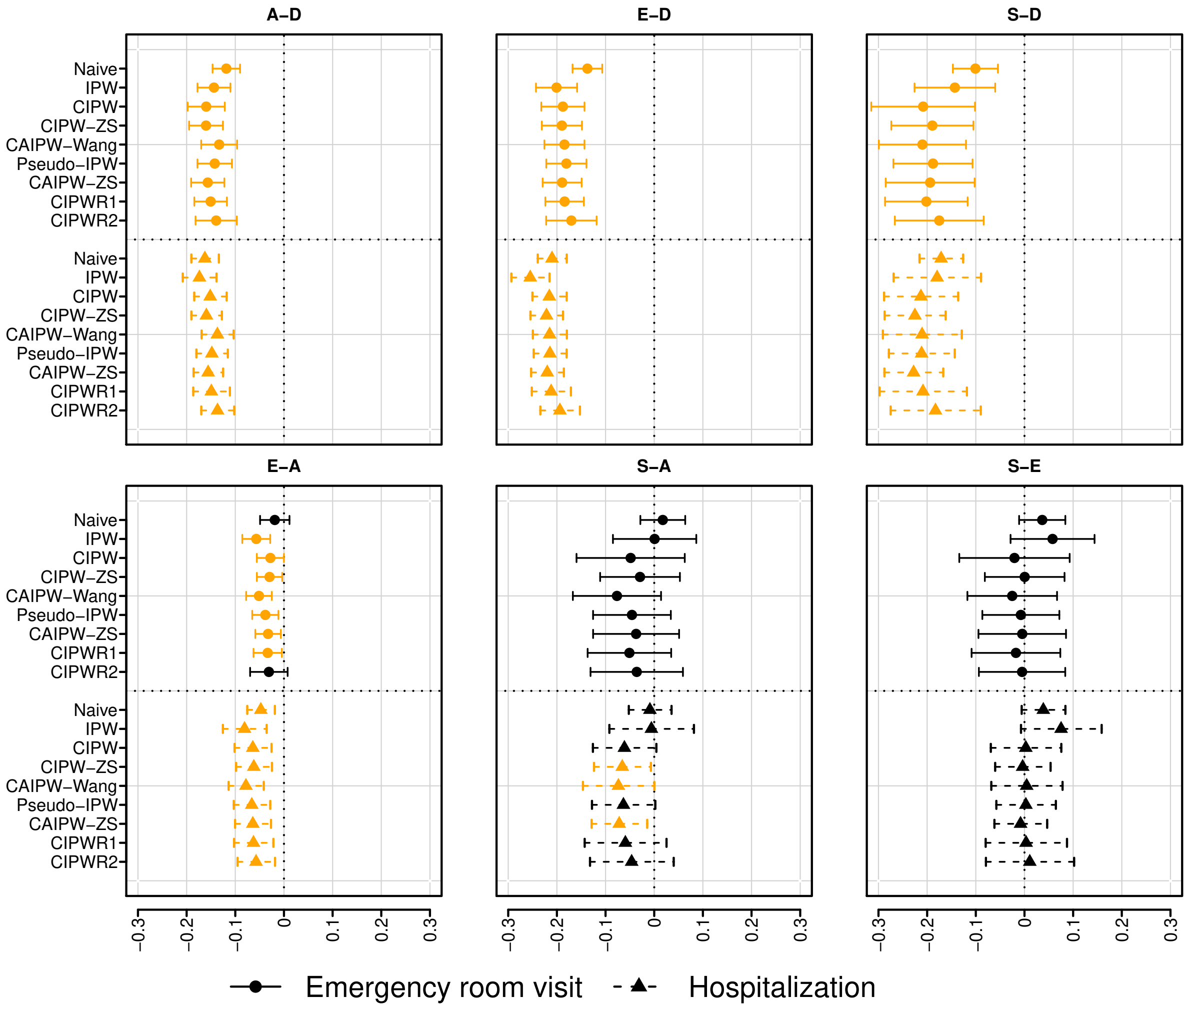


Figure B.9: Average treatment effects for ER visits and hospitalization within 270 days of treatment initiation. Data were obtained from Optum Clinformative Data Mart. Total sample size was $N = 7003$ ($N_A = 2458$, $N_D = 2162$, $N_E = 1833$, $N_S = 550$) for ER visits, and $N = 7045$ ($N_A = 2474$, $N_D = 2172$, $N_E = 1843$, $N_S = 556$) for hospitalization. CIPWR1 is based on observation time, and CIPWR2 is based on observed censoring time. Confidence intervals that exclude zero are highlighted in orange. Abbreviations: A, abiraterone; D, docetaxel; E, enzalutamide; S, sipuleucel-T; ER, emergency room visit.

# C Generation of Survival Time with Crossing Hazards

We assumed a three-phase model for the time to event $T$, and the cumulative hazard function is specified as follows:

$$\begin{aligned}\Lambda(t|X_1, X_2) = &\exp(\beta_1 X_1 + \beta_2 X_2) I(t \leq a) \\ &+ \Big\{ \frac{\exp(\beta_1 X_1 + \beta_2 X_2) b - \exp(\alpha_1 X_1 + \alpha_2 X_2) a}{b - a} \\ &- \frac{\exp(\beta_1 X_1 + \beta_2 X_2) - \exp(\alpha_1 X_1 + \alpha_2 X_2)}{b - a} t \Big\} I(a < t \leq b) \\ &+ \exp(\alpha_1 X_1 + \alpha_2 X_2) I(t > b).\end{aligned}$$

In the first scenario, $b = 0.25, a = 0.2, \beta_1 = 2, \alpha_1 = -2, \beta_2 = 0, \alpha_2 = 0$. In the sceond scenario, $b = 0.25, a = 0.2, \beta_1 = 2, \alpha_1 = 0, \beta_2 = -2, \alpha_2 = -1$. In Sections C.1 and C.2, we list the equations used to generate the event times.

## C.1 Scenario 1

Define

$$\begin{aligned}\text{termA} &= \{\exp(2X_1) - \exp(-2X_1)\}/2 \\ \text{termB} &= -\{0.25 \exp(2X_1) - 0.2 \exp(-2X_1)\} \\ \text{termC} &= -0.05 \log u + 0.02\{\exp(2X_1) - \exp(-2X_1)\}\end{aligned}$$

Then let

$$\begin{aligned}\mathcal{I}_1 &= \frac{-\log u}{\exp(2X_1)} \\ \mathcal{I}_2 &= \frac{-\text{termB} + \sqrt{\text{termB}^2 - 4\text{termA} \times \text{termC}}}{2\text{termA}} \\ \mathcal{I}_3 &= \frac{-\log u - 0.225\{\exp(2X_1) - \exp(-2X_1)\}}{\exp(-2X_1)}\end{aligned}$$

$$T' = \mathcal{I}_1 I(\mathcal{I}_1 \leq 0.2) + \mathcal{I}_2 I(\mathcal{I}_2 \leq 0.25) I(\mathcal{I}_2 > 0.2) + \mathcal{I}_3 I(\mathcal{I}_3 > 0.25)$$

The final event time was obtained using

$$T = T' I(Z = 1) + (T' + 0.1) I(Z = 2) + (T' + 0.2) I(Z = 3)$$

## C.2 Scenario 2

Define

$$\begin{aligned}\text{termA} &= \{\exp(2X_1) - \exp(-2X_1 - X_2)\}/2 \\ \text{termB} &= -\{0.25 \exp(2X_1) - 0.2 \exp(-2X_1 - X_2)\} \\ \text{termC} &= -0.05 \log u + 0.02\{\exp(2X_1) - \exp(-2X_1 - X_2)\}\end{aligned}$$

Then let

$$\mathcal{I}_1 = \frac{-\log u}{\exp(2X_1)}$$

$$\mathcal{I}_2 = \frac{-\text{termB} + \sqrt{\text{termB}^2 - 4\text{termA} \times \text{termC}}}{2\text{termA}}$$

$$\mathcal{I}_3 = \frac{-\log u - 0.225\{\exp(2X_1) - \exp(-2X_1 - X_2)\}}{\exp(-2X_1 - X_2)}$$

$$T' = \mathcal{I}_1 I(\mathcal{I}_1 \leq 0.2) + \mathcal{I}_2 I(\mathcal{I}_2 \leq 0.25) I(\mathcal{I}_2 > 0.2) + \mathcal{I}_3 I(\mathcal{I}_3 > 0.25)$$

The final event time was obtained using

$$T = T' I(Z = 1) + (T' + 0.1) I(Z = 2) + (T' + 0.15) I(Z = 3)$$
